# Supplementary material for: "Two-phase" thermodynamics of the Frenkel line
Source: arXiv:1806.07608 source file (2018-08-01)
Supplement: Supplementary file 1 [file supporting-information-two.pdf]

# Supporting Information for ‘Two-phase’ Thermodynamics of the Frenkel Line

Tae Jun Yoon,[1] Min Young Ha,[1] Won Bo Lee,[1, a)] and Youn-Woo Lee[1, b)]
*School of Chemical and Biological Engineering, Institute of Chemical Processes, Seoul National University, Seoul 08826, Republic of Korea*

This supporting information includes the calculation procedures and numerical results used in the main article. In Section I, we describe the calculation procedures. In section II, the thermodynamic data from the two-phase thermodynamics (2PT) model are presented.

## I. CALCULATION DETAILS

### A. Estimation of the critical point

The Lennard-Jones potential [Eqn. (S1)] was used to model the interaction between argon molecules ($\sigma$ = 3.405 Å and $\epsilon_{lj} = 0.238$ kcal/mol).

$$\phi(r) = 4\epsilon_{lj}\left[\left(\frac{\sigma}{r}\right)^{12} - \left(\frac{\sigma}{r}\right)^{6}\right] \tag{S1}$$

The potential was truncated and shifted at the cutoff radius of $r_{cut} = 15.0$ Å. To determine the critical point of argon, the van der Waals hypothesis was adopted, which states that $(\partial\rho/\partial p)_T$ and its first derivative become zero at the critical point.

$$\frac{\partial p}{\partial \rho} = 0; \quad \frac{\partial^2 p}{\partial \rho^2} = 0 \tag{S2}$$

NVT MD simulations were performed to obtain the system pressures at the temperatures from 150 K to 170 K and at the densities from 150 kg/m$^3$ to 200 kg/m$^3$. The timestep was $\Delta t = 0.004$ ps. The systems were equilibrated for 100,000 steps, and the pressure data were collected for additional 1,000,000 steps. Cubic equations were fitted to the pressure data. The coefficients of the determination were always larger than 0.99 ($R^2 = 0.99$). From the fitting equations, the inflection points at different temperatures were calculated. By examining the slopes of cubic equations at the inflection points, the critical temperature was obtained as the temperature at which the slope of the isotherm at the inflection point becomes zero. The critical density and the critical pressure were also obtained in the same manner. The critical temperature, pressure, and density of argon obtained are 159.14 K, 60.87 bar and 471.45 kg/m$^3$.

### B. Phase coexistence lines of argon

Vapor/liquid equilibrium line was calculated using the correlation suggested by Tanttila[1]. The equations are given as:

$$1 + x_l^3 = \frac{1}{1+t}\exp\left(\frac{\alpha t}{1+t}\right) \tag{S3a}$$

$$1 - x_g^3 = \frac{1}{1-t}\exp\left(\frac{-\alpha t}{1-t}\right) \tag{S3b}$$

where $x_i$ is $(\rho_i - \rho_c)/\rho_c$ ($i$ = gas, liquid), and $t$ is $(T_c - T)/T_c$. $\alpha = 6.6$ was used to draw the coexistence line. The liquid-solid coexistence densities of argon modeled with the Lennard-Jones potential were obtained from the correlation proposed by Heyes and Brańka[2]. The melting line was calculated as:

$$\rho_m = a + b\kappa + c\kappa^2 + d\kappa^3 + e\kappa^4 + f\kappa^6 \tag{S4}$$

where $\kappa$ is log(T) and the coefficients $a, b, c, d, e$, and $f$ are given as 0.915647, 0.196747, $0.132455 \times 10^{-1}$, $0.663076 \times 10^{-2}$, $-0.573814 \times 10^{-3}$ and $1.10827 \times 10^{-5}$.

### C. Details of the two-phase thermodynamics model

The density of states ($\Psi(\nu)$) of a system is defined as the distribution of normal modes of vibration of a system. Hence, an integration of $\Psi(\nu)$ from zero to infinity yields the total number of degree of freedom of the N particle system.

$$\int_0^\infty \Psi(\nu)d\nu = 3N \tag{S5}$$

In perfect gas, the overlap of balls is allowed. Hence, the translation of particles, which can be regarded as the oscillatory motion whose vibrational frequency is zero, is not hampered by their neighbors. In real gases, the density of states exponentially decays as the vibrational frequency of a motion increases. In stationary solid phase, on the contrary, $\Psi(\nu)$ has at least one local maximum at a specific frequency. Lin et al. (2003)[3] introduced two hypotheses to split the density of states into gas-like and solid-like contributions. They first assumed that the diffusive motion of particles entirely originates from the gas-like contribution. Second, Lin et al. (2003) hypothesized that the gas-like component could be modeled as a hard sphere system. To relate the hard sphere theory and the diffusivity, they introduced a concept of fluidicity ($f_g$), which is defined as:

$$f_g = \frac{\int_0^\infty \Psi^g(\nu)d\nu}{\int_0^\infty \Psi(\nu)d\nu} = \frac{D(T,\rho)}{D_0^{hs}(T,\rho;\sigma^{hs})} \tag{S6}$$

a) Electronic mail: wblee@snu.ac.kr
b) Electronic mail: ywlee@snu.ac.kr

where $D_0^{hs}$ term could be calculated using the Carnahan-Starling equation of state[4]. $D(T,\rho)$ is obtained from the MD simulations. Thus, the fluidicity of a system is computed by:

$$2\Delta^{-9/2} f_g^{15/2} - 6\Delta^{-3} f_g^5 - \Delta^{-3/2} f_g^{7/2} + 6\Delta^{-3/2} f_g^{5/2} + 2f_g - 2 = 0 \tag{S7}$$

where $\Delta$ is a normalized diffusivity constant calculated from the following equation.

$$\Delta = \frac{2\Psi(0)}{9N} \frac{\pi k_B T}{m}^{1/2} \rho^{1/3} (6/\pi)^{2/3} \tag{S8}$$

where $\rho$ is the bulk density of a system ($\rho = N/V$). After the fluidicity calculation, the non-rigid (gas-like) contribution to $\Psi(\nu)$ can be calculated as:

$$\Psi^g(\nu) = \frac{\Psi(0)}{1 + \left[\frac{\pi\Psi(0)\nu}{6 f_g N}\right]^2} \tag{S9}$$

The rigid (solid-like) contribution to the total density of states is $\Psi^s(\nu) = \Psi(\nu) - \Psi^g(\nu)$. After the gas-like and solid-like density of states are obtained, energy (E) and entropy (S) of a system are calculated as a linear combination of gas-like and solid-like contributions.

$$E = V_0 + \int_0^\infty [\Psi^g(\nu) W_E^g(\nu) + \Psi^s(\nu) W_E^s(\nu)] d\nu \tag{S10a}$$

$$S = \int_0^\infty [\Psi^g(\nu) W_S^g(\nu) + \Psi^s(\nu) W_S^s(\nu)] d\nu \tag{S10b}$$

Here, the weighting functions $W_Q^p$ ($Q = E, S$ and $p = g, s$) are given by:

$$W_E^g(\nu) = 0.5 \tag{S11a}$$

$$W_S^g(\nu) = \frac{1}{3}\left(\frac{5}{2} + log\left[\left(\frac{2\pi m k_B T}{h^2}\right)^{3/2} \frac{V}{f_g N}\right]\right) \tag{S11b}$$

$$W_E^s(\nu) = \frac{\theta}{2} + \frac{\theta}{e^\theta - 1} \tag{S11c}$$

$$W_S^s(\nu) = \frac{\theta}{e^\theta - 1} - log(1 - e^{-\theta}) \tag{S11d}$$

where $h$ is the Planck constant and $\theta$ is $h\nu/k_B T$. The reference energy is defined as the potential energy of a system when all oscillators (atoms) are standing still and represented as:

$$V_0 = E^{MD} - 3N(1 - 0.5 f_g)/(k_B T) \tag{S12}$$

## II. CALCULATION RESULTS

### A. Finite size-effect and the finite timestep effect

We performed two sets of the MD simulations to examine the influence of the system size and the timestep size.

TABLE S1. Solidicity data obtained using 2,000 atoms and 16,000 atoms at $T_r = 1.0$.

| $\rho\sigma^3$ | $f_s$ (2,000 atoms) | $f_s'$ (16,000 atoms) |
|---|---|---|
| 0.056 | 0.093 | 0.092 |
| 0.168 | 0.186 | 0.188 |
| 0.281 | 0.259 | 0.255 |
| 0.393 | 0.314 | 0.310 |
| 0.505 | 0.376 | 0.371 |
| 0.617 | 0.447 | 0.432 |
| 0.729 | 0.512 | 0.510 |
| 0.842 | 0.608 | 0.602 |
| 0.954 | 0.705 | 0.700 |

In the first set, the finite-size effect on the 2PT calculation results was examined by performing MD simulations with 16,000 atoms at the temperature of $T_r = 1.0$. Table S1 shows the solidicity data obtained from the MD simulations with 16,000 atoms and 2,000 atoms. It showed no significant dependence on the number of molecules in a system. In the second set, the timestep was changed from 0.002 ps to 0.001 ps and 0.0005 ps in MD simulations with 2,000 atoms at the temperature of $T_r = 70.0$. Table S2 shows the solidicity obtained from these MD simulations and the deviation from the simulations performed with the timestep of $\Delta t = 0.002$ps. No considerable dependence on the timestep was observed. Thus, both of the finite-size effect and the finite timestep effect were negligible as Lin et al. (2003) originally stated.

### B. Estimation of the crossover densities

Three crossover densities suggested in the letter are obtained as follows (Table S3). First, the inflection point of a solidicity curve is obtained by fitting a two-exponential model to the solidicity data.

$$f_s = a \exp(b\rho) - c \exp(-d\rho) \tag{S13}$$

The inflection densities of the soft-sphere and the hard-sphere fluids were followingly calculated as $\rho_{inf} = \log(cd^2/ab^2)/(b+d)$. For the soft-sphere models ($n < 20$), the crossover densities from the isofluidicity criterion ($f_s = 0.33$) were obtained by solving the fitting equation [Eqn. (S13)] numerically. The crossover densities from the energetic criterion ($E^g = E^s$) were computed by linearly interpolating the gas-like and solid-like energy data near the point of intersection.

### C. Two-phase thermodynamics calculations

Tables S8-S11 show the 2PT calculation results of argon and the fluids modeled with the repulsive $n-6$ potential ($n = 8$ and $n = 16$). In the Tables S8-S11, all thermodynamic variables are represented as the dimensionless ones. Dimensionless energy and entropy are defined

TABLE S2. Solidicity data obtained from different timesteps at $T_r = 70.0$.

| $\rho\sigma^3$ | $f_s''$ ($\Delta t = 0.001$ps) | $f_s'''$ ($\Delta t = 0.0005$ps) |
|---|---|---|
| 0.056 | 0.029 | 0.034 |
| 0.168 | 0.079 | 0.080 |
| 0.281 | 0.123 | 0.121 |
| 0.393 | 0.157 | 0.156 |
| 0.505 | 0.187 | 0.188 |
| 0.617 | 0.212 | 0.220 |
| 0.729 | 0.244 | 0.249 |
| 0.842 | 0.266 | 0.275 |
| 0.954 | 0.293 | 0.299 |
| 1.066 | 0.324 | 0.324 |
| 1.178 | 0.339 | 0.342 |
| 1.291 | 0.372 | 0.370 |
| 1.403 | 0.394 | 0.387 |
| 1.515 | 0.428 | 0.427 |
| 1.627 | 0.458 | 0.455 |
| 1.740 | 0.484 | 0.486 |
| 1.852 | 0.511 | 0.521 |
| 1.964 | 0.549 | 0.550 |
| 2.076 | 0.574 | 0.577 |
| 2.188 | 0.610 | 0.605 |
| 2.301 | 0.644 | 0.639 |
| 2.413 | 0.684 | 0.665 |
| 2.525 | 0.717 | 0.715 |

as $E^* = E/(Nk_BT)$ and $S^* = S/(Nk_B)$. The dimensionless temperatures are defined as $T^* = k_BT/\epsilon_{lj}$ where $\epsilon_{lj}$ is the energy parameter of argon. As shown in the Tables S8 and S10, the solidicities of the fluid modeled with the repulsive 12-6 potential at $T_r = 1.0$ was always similar to those of the Lennard-Jones fluids except at $T_r = 1.0$. At $T_r = 1.0$, the solidicites of the repulsive 12-6 fluids were slightly lower than that modeled with the Lennard-Jones potential because the kinetic energy of a molecule was not high enough to overcome the attractive interactions. Hence, this result substantiates that the dynamic behavior of dense supercritical fluids at high temperature is not significantly affected by the existence of the attractive interaction as the hard sphere paradigm states. Tables S4-S7 show the solidicity data of the repulsive $n-6$ fluids ($n > 20$) and the hard-sphere fluids. Because the Quasi-Crystalline Approximation (QCA) fails for these models, the solidicity data are only presented.


[1]Tantilla, W. H. Liquid-Gas Coexistence Equation. *Ph. Transit.* **1983**, *3* (4), 309-315.

[2]Heyes, D. M.; Brańka, A. C. The Lennard-Jones Melting Line and Isomorphism. *J. Chem. Phys.*, **2015**, *143* (23), 234504.

[3]Lin, S.-T.; Blanco, M.; Goddard III, W. A. The Two-Phase Model for Calculating Thermodynamic Properties of Liquids from Molecular Dynamics: Validation for the Phase Diagram of Lennard-Jones Fluids. *J. Chem. Phys.*, **2003**, *119* (22), 11792-11805.

[4]Carnahan, N. F.; Starling, K. E. Thermodynamic Properties of a Rigid-Sphere Fluid. *J. Chem. Phys.*, **1970**, *53* (2), 600-603.


TABLE S3. Two-exponential model parameters for the solidicity data and the inflection points.

| Lennard-Jones potential | | | | | | |
|---|---|---|---|---|---|---|
| $T_r$ | a | b | c | d | $\rho_{r,inf}$ | $f_{s,inf}$ |
| 1.00 | 0.195 | 0.377 | 0.167 | 1.765 | 1.368 | 0.312 |
| 5.00 | 0.209 | 0.256 | 0.197 | 0.876 | 2.124 | 0.328 |
| 10.0 | 0.222 | 0.207 | 0.213 | 0.667 | 2.628 | 0.345 |
| 30.0 | 0.223 | 0.160 | 0.212 | 0.523 | 3.400 | 0.348 |
| 50.0 | 0.213 | 0.146 | 0.208 | 0.539 | 3.773 | 0.342 |
| 70.0 | 0.222 | 0.131 | 0.212 | 0.429 | 4.168 | 0.347 |
| Repulsive 28-6 potential | | | | | | |
| $k_BT/\epsilon_{lj}$ | a | b | c | d | $\rho_{inf}\sigma^3$ | $f_{s,inf}$ |
| 1.328 | 0.173 | 1.590 | 0.162 | 8.432 | 0.326 | 0.280 |
| 6.642 | 0.182 | 1.368 | 0.172 | 5.581 | 0.397 | 0.294 |
| 13.284 | 0.181 | 1.268 | 0.175 | 5.188 | 0.431 | 0.295 |
| 39.853 | 0.215 | 1.008 | 0.187 | 2.520 | 0.479 | 0.293 |
| 66.421 | 0.184 | 1.069 | 0.179 | 4.177 | 0.513 | 0.298 |
| 92.989 | 0.181 | 1.046 | 0.178 | 4.248 | 0.527 | 0.294 |
| Repulsive 24-6 potential | | | | | | |
| $k_BT/\epsilon_{lj}$ | a | b | c | d | $\rho_{inf}\sigma^3$ | $f_{s,inf}$ |
| 1.328 | 0.175 | 1.576 | 0.166 | 7.657 | 0.336 | 0.285 |
| 6.642 | 0.181 | 1.329 | 0.137 | 5.605 | 0.375 | 0.281 |
| 13.284 | 0.178 | 1.249 | 0.173 | 4.851 | 0.440 | 0.288 |
| 39.853 | 0.178 | 1.096 | 0.183 | 4.479 | 0.510 | 0.292 |
| 66.421 | 0.185 | 0.998 | 0.186 | 3.840 | 0.557 | 0.302 |
| 92.989 | 0.173 | 1.012 | 0.175 | 4.278 | 0.547 | 0.284 |
| Repulsive 20-6 potential | | | | | | |
| $k_BT/\epsilon_{lj}$ | a | b | c | d | $\rho_{inf}\sigma^3$ | $f_{s,inf}$ |
| 1.328 | 0.180 | 1.511 | 0.165 | 6.144 | 0.355 | 0.290 |
| 6.642 | 0.185 | 1.256 | 0.175 | 5.025 | 0.433 | 0.299 |
| 13.284 | 0.179 | 1.187 | 0.160 | 5.123 | 0.446 | 0.287 |
| 39.853 | 0.187 | 0.975 | 0.178 | 3.694 | 0.560 | 0.300 |
| 66.421 | 0.190 | 0.895 | 0.179 | 3.262 | 0.607 | 0.303 |
| 92.989 | 0.186 | 0.865 | 0.177 | 3.189 | 0.632 | 0.298 |
| Repulsive 16-6 potential | | | | | | |
| $k_BT/\epsilon_{lj}$ | a | b | c | d | $\rho_{inf}\sigma^3$ | $f_{s,inf}$ |
| 1.328 | 0.181 | 1.479 | 0.166 | 6.106 | 0.362 | 0.291 |
| 6.642 | 0.184 | 1.166 | 0.171 | 4.220 | 0.464 | 0.292 |
| 13.284 | 0.188 | 1.022 | 0.178 | 3.983 | 0.533 | 0.303 |
| 39.853 | 0.185 | 0.853 | 0.181 | 3.393 | 0.645 | 0.300 |
| 66.421 | 0.201 | 0.732 | 0.193 | 2.443 | 0.747 | 0.315 |
| 92.989 | 0.200 | 0.690 | 0.191 | 2.305 | 0.791 | 0.314 |
| Repulsive 12-6 potential | | | | | | |
| $k_BT/\epsilon_{lj}$ | a | b | c | d | $\rho_{inf}\sigma^3$ | $f_{s,inf}$ |
| 1.328 | 0.174 | 1.431 | 0.168 | 5.995 | 0.381 | 0.283 |
| 6.642 | 0.197 | 0.954 | 0.199 | 3.690 | 0.585 | 0.321 |
| 13.284 | 0.210 | 0.776 | 0.202 | 2.599 | 0.705 | 0.331 |
| 39.853 | 0.214 | 0.592 | 0.206 | 1.994 | 0.924 | 0.337 |
| 66.421 | 0.214 | 0.521 | 0.208 | 1.871 | 1.058 | 0.342 |
| 92.989 | 0.207 | 0.496 | 0.200 | 1.754 | 1.106 | 0.330 |
| Repulsive 8-6 potential | | | | | | |
| $k_BT/\epsilon_{lj}$ | a | b | c | d | $\rho_{inf}\sigma^3$ | $f_{s,inf}$ |
| 1.328 | 0.217 | 0.918 | 0.203 | 3.203 | 0.590 | 0.342 |
| 6.642 | 0.215 | 0.574 | 0.210 | 2.242 | 0.961 | 0.348 |
| 13.284 | 0.211 | 0.464 | 0.207 | 1.962 | 1.180 | 0.344 |
| 39.853 | 0.216 | 0.315 | 0.213 | 1.377 | 1.736 | 0.353 |
| 66.421 | 0.210 | 0.270 | 0.208 | 1.249 | 2.010 | 0.344 |
| 92.989 | 0.213 | 0.237 | 0.212 | 1.099 | 2.293 | 0.349 |
| Hard-sphere potential | | | | | | |
| $T^*$ | a | b | c | d | $\rho_{inf}\sigma^3$ | $f_{s,inf}$ |
| 1.000 | 0.166 | 1.614 | 0.271 | 10.95 | 0.344 | 0.282 |

TABLE S4: Solidicity of the fluids modeled with $n = 20$.

| $T^*(= k_BT/\epsilon_{lj})$ | $\rho\sigma^3$ | $f_s$ |
|---|---|---|
| 1.328 | 0.056 | 0.004 |
| 1.328 | 0.168 | 0.171 |
| 1.328 | 0.281 | 0.250 |
| 1.328 | 0.393 | 0.307 |
| 1.328 | 0.505 | 0.385 |
| 1.328 | 0.617 | 0.453 |
| 1.328 | 0.729 | 0.542 |
| 1.328 | 0.842 | 0.639 |
| 1.328 | 0.954 | 0.765 |
| 6.642 | 0.056 | 0.067 |
| 6.642 | 0.168 | 0.149 |
| 6.642 | 0.281 | 0.224 |
| 6.642 | 0.393 | 0.281 |
| 6.642 | 0.505 | 0.331 |
| 6.642 | 0.617 | 0.395 |
| 6.642 | 0.729 | 0.454 |
| 6.642 | 0.842 | 0.531 |
| 6.642 | 0.954 | 0.613 |
| 6.642 | 1.066 | 0.703 |
| 13.284 | 0.056 | 0.073 |
| 13.284 | 0.168 | 0.145 |
| 13.284 | 0.281 | 0.210 |
| 13.284 | 0.393 | 0.270 |
| 13.284 | 0.505 | 0.317 |
| 13.284 | 0.617 | 0.367 |
| 13.284 | 0.729 | 0.416 |
| 13.284 | 0.842 | 0.482 |
| 13.284 | 0.954 | 0.551 |
| 13.284 | 1.066 | 0.637 |
| 39.853 | 0.056 | 0.053 |
| 39.853 | 0.168 | 0.124 |
| 39.853 | 0.281 | 0.179 |
| 39.853 | 0.393 | 0.237 |
| 39.853 | 0.505 | 0.285 |
| 39.853 | 0.617 | 0.318 |
| 39.853 | 0.729 | 0.365 |
| 39.853 | 0.842 | 0.415 |
| 39.853 | 0.954 | 0.470 |
| 39.853 | 1.066 | 0.525 |
| 39.853 | 1.178 | 0.594 |
| 39.853 | 1.291 | 0.653 |
| 39.853 | 1.403 | 0.734 |
| 39.853 | 1.515 | 0.816 |
| 66.421 | 0.056 | 0.051 |
| 66.421 | 0.168 | 0.119 |
| 66.421 | 0.281 | 0.168 |
| 66.421 | 0.393 | 0.225 |
| 66.421 | 0.505 | 0.268 |
| 66.421 | 0.617 | 0.304 |
| 66.421 | 0.729 | 0.342 |
| 66.421 | 0.842 | 0.394 |
| 66.421 | 0.954 | 0.435 |
| 66.421 | 1.066 | 0.494 |
| 66.421 | 1.178 | 0.542 |
| 66.421 | 1.291 | 0.599 |
| 66.421 | 1.403 | 0.660 |
| 66.421 | 1.515 | 0.739 |
| 66.421 | 1.627 | 0.821 |
| 92.989 | 0.056 | 0.046 |
| 92.989 | 0.168 | 0.113 |
| 92.989 | 0.281 | 0.163 |
| 92.989 | 0.393 | 0.215 |
| 92.989 | 0.505 | 0.255 |
| 92.989 | 0.617 | 0.284 |
| 92.989 | 0.729 | 0.333 |
| 92.989 | 0.842 | 0.371 |
| 92.989 | 0.954 | 0.416 |
| 92.989 | 1.066 | 0.462 |
| 92.989 | 1.178 | 0.519 |
| 92.989 | 1.291 | 0.564 |
| 92.989 | 1.403 | 0.621 |
| 92.989 | 1.515 | 0.691 |
| 92.989 | 1.627 | 0.757 |

TABLE S5: Solidicity of the fluids modeled with $n = 24$.

| $T^*(= k_BT/\epsilon_{lj})$ | $\rho\sigma^3$ | $f_s$ |
|---|---|---|
| 1.328 | 0.056 | 0.084 |
| 1.328 | 0.168 | 0.180 |
| 1.328 | 0.281 | 0.255 |
| 1.328 | 0.393 | 0.316 |
| 1.328 | 0.505 | 0.386 |
| 1.328 | 0.617 | 0.468 |
| 1.328 | 0.729 | 0.549 |
| 1.328 | 0.842 | 0.650 |
| 1.328 | 0.954 | 0.793 |
| 6.642 | 0.056 | 0.095 |
| 6.642 | 0.168 | 0.174 |
| 6.642 | 0.281 | 0.231 |
| 6.642 | 0.393 | 0.292 |
| 6.642 | 0.505 | 0.346 |
| 6.642 | 0.617 | 0.406 |
| 6.642 | 0.729 | 0.476 |
| 6.642 | 0.842 | 0.555 |
| 6.642 | 0.954 | 0.642 |
| 6.642 | 1.066 | 0.739 |
| 13.284 | 0.056 | 0.060 |
| 13.284 | 0.168 | 0.144 |
| 13.284 | 0.281 | 0.206 |
| 13.284 | 0.393 | 0.268 |
| 13.284 | 0.505 | 0.321 |
| 13.284 | 0.617 | 0.377 |
| 13.284 | 0.729 | 0.439 |
| 13.284 | 0.842 | 0.500 |
| 13.284 | 0.954 | 0.592 |
| 13.284 | 1.066 | 0.672 |
| 39.853 | 0.056 | 0.048 |
| 39.853 | 0.168 | 0.125 |
| 39.853 | 0.281 | 0.187 |
| 39.853 | 0.393 | 0.248 |
| 39.853 | 0.505 | 0.293 |
| 39.853 | 0.617 | 0.334 |
| 39.853 | 0.729 | 0.387 |
| 39.853 | 0.842 | 0.445 |
| 39.853 | 0.954 | 0.504 |
| 39.853 | 1.066 | 0.571 |
| 39.853 | 1.178 | 0.641 |
| 39.853 | 1.291 | 0.734 |
| 66.421 | 0.056 | 0.045 |
| 66.421 | 0.168 | 0.124 |
| 66.421 | 0.281 | 0.183 |
| 66.421 | 0.393 | 0.233 |

| | | |
|---|---|---|
| 66.421 | 0.505 | 0.280 |
| 66.421 | 0.617 | 0.322 |
| 66.421 | 0.729 | 0.375 |
| 66.421 | 0.842 | 0.424 |
| 66.421 | 0.954 | 0.473 |
| 66.421 | 1.066 | 0.533 |
| 66.421 | 1.178 | 0.603 |
| 66.421 | 1.291 | 0.676 |
| 66.421 | 1.403 | 0.749 |
| 66.421 | 1.515 | 0.840 |
| 92.989 | 0.056 | 0.046 |
| 92.989 | 0.168 | 0.117 |
| 92.989 | 0.281 | 0.179 |
| 92.989 | 0.393 | 0.225 |
| 92.989 | 0.505 | 0.268 |
| 92.989 | 0.617 | 0.311 |
| 92.989 | 0.729 | 0.351 |
| 92.989 | 0.842 | 0.403 |
| 92.989 | 0.954 | 0.459 |
| 92.989 | 1.066 | 0.507 |
| 92.989 | 1.178 | 0.574 |
| 92.989 | 1.291 | 0.630 |
| 92.989 | 1.403 | 0.715 |
| 92.989 | 1.515 | 0.788 |
| 92.989 | 1.627 | 0.911 |

TABLE S6: Solidicity of the fluids modeled with $n = 28$.

| $T^*(= k_B T/\epsilon_{lj})$ | $\rho\sigma^3$ | $f_s$ |
|---|---|---|
| 1.328 | 0.056 | 0.109 |
| 1.328 | 0.168 | 0.194 |
| 1.328 | 0.281 | 0.265 |
| 1.328 | 0.393 | 0.331 |
| 1.328 | 0.505 | 0.392 |
| 1.328 | 0.617 | 0.463 |
| 1.328 | 0.729 | 0.549 |
| 1.328 | 0.842 | 0.657 |
| 1.328 | 0.954 | 0.801 |
| 6.642 | 0.056 | 0.072 |
| 6.642 | 0.168 | 0.159 |
| 6.642 | 0.281 | 0.225 |
| 6.642 | 0.393 | 0.299 |
| 6.642 | 0.505 | 0.358 |
| 6.642 | 0.617 | 0.421 |
| 6.642 | 0.729 | 0.480 |
| 6.642 | 0.842 | 0.578 |
| 6.642 | 0.954 | 0.665 |
| 6.642 | 1.066 | 0.777 |
| 13.284 | 0.056 | 0.063 |
| 13.284 | 0.168 | 0.153 |
| 13.284 | 0.281 | 0.214 |
| 13.284 | 0.393 | 0.281 |
| 13.284 | 0.505 | 0.328 |
| 13.284 | 0.617 | 0.389 |
| 13.284 | 0.729 | 0.452 |
| 13.284 | 0.842 | 0.532 |
| 13.284 | 0.954 | 0.602 |
| 13.284 | 1.066 | 0.701 |
| 39.853 | 0.056 | 0.060 |
| 39.853 | 0.168 | 0.134 |
| 39.853 | 0.281 | 0.203 |
| 39.853 | 0.393 | 0.260 |
| 39.853 | 0.505 | 0.306 |
| 39.853 | 0.617 | 0.352 |
| 39.853 | 0.729 | 0.416 |
| 39.853 | 0.842 | 0.466 |
| 39.853 | 0.954 | 0.544 |
| 39.853 | 1.066 | 0.614 |
| 39.853 | 1.178 | 0.698 |
| 39.853 | 1.291 | 0.803 |
| 39.853 | 1.403 | 0.910 |
| 66.421 | 0.056 | 0.056 |
| 66.421 | 0.168 | 0.125 |
| 66.421 | 0.281 | 0.202 |
| 66.421 | 0.393 | 0.245 |
| 66.421 | 0.505 | 0.292 |
| 66.421 | 0.617 | 0.342 |
| 66.421 | 0.729 | 0.391 |
| 66.421 | 0.842 | 0.455 |
| 66.421 | 0.954 | 0.508 |
| 66.421 | 1.066 | 0.573 |
| 66.421 | 1.178 | 0.647 |
| 66.421 | 1.291 | 0.731 |
| 66.421 | 1.403 | 0.827 |
| 92.989 | 0.056 | 0.053 |
| 92.989 | 0.168 | 0.123 |
| 92.989 | 0.281 | 0.189 |
| 92.989 | 0.393 | 0.239 |
| 92.989 | 0.505 | 0.290 |
| 92.989 | 0.617 | 0.326 |
| 92.989 | 0.729 | 0.386 |
| 92.989 | 0.842 | 0.432 |
| 92.989 | 0.954 | 0.490 |
| 92.989 | 1.066 | 0.548 |
| 92.989 | 1.178 | 0.608 |
| 92.989 | 1.291 | 0.696 |
| 92.989 | 1.403 | 0.790 |

TABLE S7: Solidicity data of the hard-sphere fluid.

| $T^*$ | $\rho\sigma^3$ | $f_s$ |
|---|---|---|
| 1.000 | 0.115 | 0.123 |
| 1.000 | 0.229 | 0.214 |
| 1.000 | 0.344 | 0.285 |
| 1.000 | 0.458 | 0.351 |
| 1.000 | 0.573 | 0.426 |
| 1.000 | 0.688 | 0.494 |
| 1.000 | 0.802 | 0.597 |
| 1.000 | 0.917 | 0.722 |
| 1.000 | 1.031 | 0.883 |

TABLE S8: Thermodynamic calculation results of argon

| $k_BT/\epsilon_{lj}$ | $\rho\sigma^3$ | $f_s$ | $E^{*,MD}$ | $E^{*,,tot}$ | $E^{*,g}$ | $E^{*,s}$ | $V_0^*$ | $S^{*,tot}$ | $S^{*,g}$ | $S^{*,s}$ |
|---|---|---|---|---|---|---|---|---|---|---|
| 1.328 | 0.056 | 0.093 | 1.180 | 1.171 | 1.360 | 0.279 | -0.468 | 13.582 | 12.423 | 1.159 |
| 1.328 | 0.168 | 0.186 | 0.561 | 0.507 | 1.220 | 0.528 | -1.241 | 12.112 | 10.327 | 1.785 |
| 1.328 | 0.281 | 0.259 | 0.013 | -0.071 | 1.110 | 0.732 | -1.913 | 11.337 | 9.071 | 2.266 |
| 1.328 | 0.393 | 0.314 | -0.494 | -0.572 | 1.028 | 0.886 | -2.486 | 10.745 | 8.199 | 2.547 |
| 1.328 | 0.505 | 0.376 | -0.991 | -1.079 | 0.934 | 1.062 | -3.075 | 10.247 | 7.326 | 2.921 |
| 1.328 | 0.617 | 0.447 | -1.517 | -1.613 | 0.828 | 1.264 | -3.706 | 9.713 | 6.408 | 3.306 |
| 1.328 | 0.729 | 0.512 | -2.029 | -2.136 | 0.731 | 1.454 | -4.321 | 9.034 | 5.581 | 3.453 |
| 1.328 | 0.842 | 0.608 | -2.462 | -2.571 | 0.586 | 1.742 | -4.900 | 8.284 | 4.408 | 3.876 |
| 1.328 | 0.954 | 0.705 | -2.723 | -2.822 | 0.441 | 2.041 | -5.304 | 7.414 | 3.229 | 4.185 |
| 6.642 | 0.056 | 0.051 | 1.462 | 1.461 | 1.423 | 0.153 | -0.115 | 16.247 | 15.251 | 0.996 |
| 6.642 | 0.168 | 0.131 | 1.390 | 1.386 | 1.303 | 0.388 | -0.305 | 15.166 | 13.084 | 2.082 |
| 6.642 | 0.281 | 0.193 | 1.323 | 1.315 | 1.210 | 0.572 | -0.467 | 14.494 | 11.784 | 2.711 |
| 6.642 | 0.393 | 0.241 | 1.262 | 1.254 | 1.137 | 0.716 | -0.599 | 13.892 | 10.849 | 3.043 |
| 6.642 | 0.505 | 0.290 | 1.214 | 1.203 | 1.064 | 0.860 | -0.720 | 13.367 | 10.005 | 3.362 |
| 6.642 | 0.617 | 0.327 | 1.184 | 1.172 | 1.008 | 0.970 | -0.805 | 12.832 | 9.367 | 3.465 |
| 6.642 | 0.729 | 0.383 | 1.185 | 1.171 | 0.922 | 1.139 | -0.891 | 12.407 | 8.494 | 3.913 |
| 6.642 | 0.842 | 0.435 | 1.228 | 1.214 | 0.845 | 1.293 | -0.924 | 11.948 | 7.716 | 4.231 |
| 6.642 | 0.954 | 0.488 | 1.330 | 1.317 | 0.765 | 1.451 | -0.900 | 11.437 | 6.938 | 4.498 |
| 6.642 | 1.066 | 0.548 | 1.508 | 1.500 | 0.674 | 1.634 | -0.808 | 10.935 | 6.060 | 4.875 |
| 6.642 | 1.178 | 0.607 | 1.784 | 1.783 | 0.586 | 1.810 | -0.613 | 10.376 | 5.224 | 5.152 |
| 6.642 | 1.291 | 0.680 | 2.183 | 2.197 | 0.476 | 2.031 | -0.310 | 9.770 | 4.183 | 5.587 |
| 6.642 | 1.403 | 0.745 | 2.736 | 2.768 | 0.379 | 2.229 | 0.161 | 9.117 | 3.253 | 5.864 |
| 13.284 | 0.056 | 0.043 | 1.488 | 1.488 | 1.435 | 0.129 | -0.077 | 17.202 | 16.371 | 0.831 |
| 13.284 | 0.168 | 0.113 | 1.469 | 1.467 | 1.330 | 0.336 | -0.199 | 16.182 | 14.261 | 1.920 |
| 13.284 | 0.281 | 0.161 | 1.458 | 1.452 | 1.258 | 0.479 | -0.285 | 15.486 | 13.097 | 2.389 |
| 13.284 | 0.393 | 0.212 | 1.452 | 1.447 | 1.181 | 0.631 | -0.365 | 15.044 | 12.069 | 2.975 |
| 13.284 | 0.505 | 0.255 | 1.460 | 1.452 | 1.116 | 0.759 | -0.423 | 14.577 | 11.251 | 3.326 |
| 13.284 | 0.617 | 0.306 | 1.482 | 1.475 | 1.039 | 0.912 | -0.476 | 14.221 | 10.361 | 3.860 |
| 13.284 | 0.729 | 0.346 | 1.528 | 1.518 | 0.979 | 1.030 | -0.492 | 13.781 | 9.677 | 4.104 |
| 13.284 | 0.842 | 0.375 | 1.601 | 1.591 | 0.935 | 1.117 | -0.461 | 13.329 | 9.168 | 4.160 |
| 13.284 | 0.954 | 0.426 | 1.711 | 1.701 | 0.859 | 1.269 | -0.426 | 12.939 | 8.367 | 4.571 |
| 13.284 | 1.066 | 0.471 | 1.868 | 1.858 | 0.791 | 1.404 | -0.336 | 12.524 | 7.658 | 4.866 |
| 13.284 | 1.178 | 0.521 | 2.077 | 2.077 | 0.716 | 1.554 | -0.193 | 12.106 | 6.885 | 5.221 |
| 13.284 | 1.291 | 0.561 | 2.359 | 2.364 | 0.656 | 1.674 | 0.035 | 11.639 | 6.266 | 5.373 |
| 13.284 | 1.403 | 0.615 | 2.723 | 2.738 | 0.575 | 1.835 | 0.327 | 11.169 | 5.450 | 5.719 |
| 13.284 | 1.515 | 0.680 | 3.184 | 3.212 | 0.477 | 2.031 | 0.703 | 10.656 | 4.468 | 6.189 |
| 13.284 | 1.627 | 0.731 | 3.767 | 3.807 | 0.400 | 2.187 | 1.221 | 10.121 | 3.686 | 6.435 |
| 39.853 | 0.056 | 0.035 | 1.505 | 1.504 | 1.448 | 0.105 | -0.048 | 18.935 | 18.095 | 0.841 |
| 39.853 | 0.168 | 0.093 | 1.518 | 1.519 | 1.359 | 0.281 | -0.121 | 17.951 | 16.047 | 1.904 |
| 39.853 | 0.281 | 0.137 | 1.537 | 1.538 | 1.293 | 0.413 | -0.168 | 17.305 | 14.863 | 2.442 |
| 39.853 | 0.393 | 0.182 | 1.563 | 1.563 | 1.225 | 0.548 | -0.210 | 16.910 | 13.842 | 3.068 |
| 39.853 | 0.505 | 0.214 | 1.597 | 1.600 | 1.178 | 0.643 | -0.221 | 16.455 | 13.134 | 3.321 |
| 39.853 | 0.617 | 0.258 | 1.642 | 1.644 | 1.111 | 0.777 | -0.244 | 16.183 | 12.267 | 3.916 |
| 39.853 | 0.729 | 0.277 | 1.697 | 1.700 | 1.081 | 0.835 | -0.216 | 15.722 | 11.835 | 3.887 |
| 39.853 | 0.842 | 0.311 | 1.770 | 1.773 | 1.030 | 0.938 | -0.195 | 15.406 | 11.194 | 4.211 |
| 39.853 | 0.954 | 0.343 | 1.857 | 1.863 | 0.982 | 1.032 | -0.152 | 15.099 | 10.612 | 4.487 |
| 39.853 | 1.066 | 0.381 | 1.967 | 1.976 | 0.926 | 1.146 | -0.095 | 14.800 | 9.947 | 4.853 |
| 39.853 | 1.178 | 0.406 | 2.102 | 2.113 | 0.887 | 1.223 | 0.003 | 14.450 | 9.481 | 4.968 |
| 39.853 | 1.291 | 0.441 | 2.266 | 2.278 | 0.834 | 1.329 | 0.116 | 14.147 | 8.876 | 5.271 |
| 39.853 | 1.403 | 0.479 | 2.464 | 2.480 | 0.778 | 1.442 | 0.261 | 13.835 | 8.240 | 5.596 |
| 39.853 | 1.515 | 0.520 | 2.698 | 2.722 | 0.715 | 1.566 | 0.440 | 13.507 | 7.547 | 5.960 |
| 39.853 | 1.627 | 0.552 | 2.978 | 3.005 | 0.668 | 1.661 | 0.676 | 13.148 | 7.014 | 6.134 |
| 39.853 | 1.740 | 0.602 | 3.311 | 3.345 | 0.592 | 1.814 | 0.940 | 12.804 | 6.180 | 6.624 |
| 39.853 | 1.852 | 0.639 | 3.693 | 3.742 | 0.536 | 1.925 | 1.281 | 12.418 | 5.566 | 6.852 |
| 39.853 | 1.964 | 0.675 | 4.143 | 4.201 | 0.481 | 2.035 | 1.685 | 12.027 | 4.959 | 7.068 |
| 39.853 | 2.076 | 0.724 | 4.665 | 4.736 | 0.408 | 2.182 | 2.146 | 11.600 | 4.150 | 7.449 |
| 66.421 | 0.056 | 0.032 | 1.508 | 1.508 | 1.452 | 0.096 | -0.040 | 19.743 | 18.890 | 0.853 |
| 66.421 | 0.168 | 0.081 | 1.526 | 1.528 | 1.378 | 0.243 | -0.094 | 18.636 | 16.965 | 1.671 |
| 66.421 | 0.281 | 0.131 | 1.549 | 1.550 | 1.302 | 0.396 | -0.148 | 18.230 | 15.625 | 2.605 |
| 66.421 | 0.393 | 0.163 | 1.578 | 1.579 | 1.254 | 0.491 | -0.166 | 17.683 | 14.793 | 2.890 |

*Continued on next page*

TABLE S8 – Thermodynamic calculation results of argon (continued)

| $k_BT/\epsilon_{lj}$ | $\rho\sigma^3$ | $f_s$ | $E^{*,MD}$ | $E^{*,,tot}$ | $E^{*,g}$ | $E^{*,s}$ | $V_0^*$ | $S^{*,tot}$ | $S^{*,g}$ | $S^{*,s}$ |
|---|---|---|---|---|---|---|---|---|---|---|
| 66.421 | 0.505 | 0.200 | 1.614 | 1.617 | 1.198 | 0.603 | -0.184 | 17.350 | 13.963 | 3.388 |
| 66.421 | 0.617 | 0.234 | 1.657 | 1.660 | 1.147 | 0.706 | -0.192 | 17.017 | 13.234 | 3.783 |
| 66.421 | 0.729 | 0.261 | 1.710 | 1.714 | 1.105 | 0.789 | -0.180 | 16.673 | 12.647 | 4.026 |
| 66.421 | 0.842 | 0.289 | 1.775 | 1.779 | 1.063 | 0.873 | -0.157 | 16.365 | 12.082 | 4.283 |
| 66.421 | 0.954 | 0.311 | 1.850 | 1.857 | 1.030 | 0.938 | -0.112 | 16.023 | 11.637 | 4.386 |
| 66.421 | 1.066 | 0.344 | 1.942 | 1.951 | 0.980 | 1.039 | -0.067 | 15.776 | 11.015 | 4.761 |
| 66.421 | 1.178 | 0.373 | 2.049 | 2.063 | 0.936 | 1.128 | -0.001 | 15.494 | 10.466 | 5.028 |
| 66.421 | 1.291 | 0.395 | 2.178 | 2.192 | 0.903 | 1.192 | 0.097 | 15.171 | 10.059 | 5.112 |
| 66.421 | 1.403 | 0.428 | 2.330 | 2.346 | 0.853 | 1.293 | 0.200 | 14.911 | 9.462 | 5.450 |
| 66.421 | 1.515 | 0.453 | 2.505 | 2.526 | 0.815 | 1.369 | 0.342 | 14.603 | 9.003 | 5.600 |
| 66.421 | 1.627 | 0.489 | 2.710 | 2.737 | 0.761 | 1.477 | 0.499 | 14.332 | 8.378 | 5.954 |
| 66.421 | 1.740 | 0.524 | 2.948 | 2.977 | 0.708 | 1.582 | 0.687 | 14.050 | 7.771 | 6.280 |
| 66.421 | 1.852 | 0.558 | 3.222 | 3.258 | 0.657 | 1.685 | 0.917 | 13.743 | 7.180 | 6.563 |
| 66.421 | 1.964 | 0.590 | 3.535 | 3.577 | 0.608 | 1.783 | 1.186 | 13.421 | 6.615 | 6.806 |
| 66.421 | 2.076 | 0.622 | 3.894 | 3.949 | 0.560 | 1.879 | 1.510 | 13.087 | 6.061 | 7.026 |
| 66.421 | 2.188 | 0.671 | 4.301 | 4.369 | 0.487 | 2.026 | 1.856 | 12.746 | 5.230 | 7.516 |
| 66.421 | 2.301 | 0.705 | 4.765 | 4.842 | 0.435 | 2.130 | 2.277 | 12.386 | 4.631 | 7.755 |
| 66.421 | 2.413 | 0.744 | 5.287 | 5.378 | 0.377 | 2.246 | 2.755 | 12.006 | 3.969 | 8.038 |
| 92.989 | 0.056 | 0.028 | 1.507 | 1.508 | 1.458 | 0.084 | -0.034 | 20.143 | 19.453 | 0.690 |
| 92.989 | 0.168 | 0.076 | 1.528 | 1.529 | 1.385 | 0.230 | -0.086 | 19.194 | 17.507 | 1.688 |
| 92.989 | 0.281 | 0.117 | 1.553 | 1.555 | 1.322 | 0.355 | -0.123 | 18.639 | 16.303 | 2.337 |
| 92.989 | 0.393 | 0.161 | 1.582 | 1.584 | 1.257 | 0.486 | -0.159 | 18.338 | 15.249 | 3.089 |
| 92.989 | 0.505 | 0.186 | 1.618 | 1.621 | 1.218 | 0.564 | -0.161 | 17.863 | 14.588 | 3.275 |
| 92.989 | 0.617 | 0.214 | 1.661 | 1.664 | 1.176 | 0.648 | -0.160 | 17.518 | 13.952 | 3.566 |
| 92.989 | 0.729 | 0.245 | 1.711 | 1.714 | 1.129 | 0.742 | -0.156 | 17.235 | 13.288 | 3.947 |
| 92.989 | 0.842 | 0.265 | 1.771 | 1.774 | 1.098 | 0.802 | -0.127 | 16.892 | 12.841 | 4.051 |
| 92.989 | 0.954 | 0.292 | 1.840 | 1.843 | 1.057 | 0.885 | -0.099 | 16.632 | 12.284 | 4.348 |
| 92.989 | 1.066 | 0.321 | 1.920 | 1.924 | 1.013 | 0.973 | -0.062 | 16.394 | 11.718 | 4.675 |
| 92.989 | 1.178 | 0.350 | 2.017 | 2.021 | 0.970 | 1.059 | -0.008 | 16.142 | 11.166 | 4.976 |
| 92.989 | 1.291 | 0.372 | 2.129 | 2.133 | 0.937 | 1.126 | 0.071 | 15.852 | 10.737 | 5.115 |
| 92.989 | 1.403 | 0.388 | 2.259 | 2.264 | 0.911 | 1.176 | 0.176 | 15.558 | 10.403 | 5.155 |
| 92.989 | 1.515 | 0.424 | 2.409 | 2.415 | 0.857 | 1.285 | 0.272 | 15.325 | 9.750 | 5.575 |
| 92.989 | 1.627 | 0.464 | 2.577 | 2.583 | 0.797 | 1.405 | 0.381 | 15.108 | 9.043 | 6.065 |
| 92.989 | 1.740 | 0.480 | 2.777 | 2.783 | 0.773 | 1.454 | 0.557 | 14.794 | 8.732 | 6.062 |
| 92.989 | 1.852 | 0.523 | 3.001 | 3.008 | 0.709 | 1.582 | 0.717 | 14.554 | 7.982 | 6.573 |
| 92.989 | 1.964 | 0.547 | 3.256 | 3.263 | 0.671 | 1.657 | 0.935 | 14.261 | 7.534 | 6.727 |
| 92.989 | 2.076 | 0.575 | 3.547 | 3.555 | 0.629 | 1.741 | 1.185 | 13.971 | 7.036 | 6.935 |
| 92.989 | 2.188 | 0.616 | 3.875 | 3.883 | 0.567 | 1.865 | 1.451 | 13.671 | 6.313 | 7.357 |
| 92.989 | 2.301 | 0.646 | 4.244 | 4.252 | 0.522 | 1.955 | 1.775 | 13.360 | 5.782 | 7.578 |
| 92.989 | 2.413 | 0.677 | 4.658 | 4.667 | 0.475 | 2.050 | 2.143 | 13.040 | 5.229 | 7.811 |
| 92.989 | 2.525 | 0.715 | 5.123 | 5.133 | 0.419 | 2.163 | 2.551 | 12.697 | 4.568 | 8.129 |

TABLE S9: Thermodynamic calculation results of repulsive 16-6 fluid

| $k_BT/\epsilon_{lj}$ | $\rho\sigma^3$ | $f_s$ | $E^{*,MD}$ | $E^{*,,tot}$ | $E^{*,g}$ | $E^{*,s}$ | $V_0^*$ | $S^{*,tot}$ | $S^{*,g}$ | $S^{*,s}$ |
|---|---|---|---|---|---|---|---|---|---|---|
| 1.328 | 0.056 | 0.080 | 1.508 | 1.596 | 1.384 | 0.324 | -0.113 | 13.797 | 12.634 | 1.164 |
| 1.328 | 0.168 | 0.168 | 1.529 | 1.497 | 1.248 | 0.472 | -0.223 | 12.514 | 10.551 | 1.963 |
| 1.328 | 0.281 | 0.250 | 1.559 | 1.506 | 1.125 | 0.697 | -0.316 | 11.720 | 9.182 | 2.538 |
| 1.328 | 0.393 | 0.308 | 1.600 | 1.533 | 1.037 | 0.857 | -0.362 | 10.924 | 8.273 | 2.652 |
| 1.328 | 0.505 | 0.377 | 1.662 | 1.581 | 0.934 | 1.050 | -0.403 | 10.226 | 7.325 | 2.901 |
| 1.328 | 0.617 | 0.441 | 1.754 | 1.665 | 0.838 | 1.235 | -0.408 | 9.485 | 6.477 | 3.008 |
| 1.328 | 0.729 | 0.536 | 1.893 | 1.798 | 0.696 | 1.512 | -0.410 | 8.734 | 5.314 | 3.420 |
| 1.328 | 0.842 | 0.624 | 2.115 | 2.023 | 0.564 | 1.780 | -0.320 | 7.847 | 4.236 | 3.612 |
| 1.328 | 0.954 | 0.744 | 2.477 | 2.402 | 0.384 | 2.157 | -0.138 | 6.777 | 2.776 | 4.001 |
| 6.642 | 0.056 | 0.060 | 1.512 | 1.513 | 1.409 | 0.182 | -0.078 | 16.287 | 15.116 | 1.171 |
| 6.642 | 0.168 | 0.142 | 1.542 | 1.534 | 1.287 | 0.417 | -0.170 | 15.157 | 12.931 | 2.226 |
| 6.642 | 0.281 | 0.201 | 1.583 | 1.571 | 1.197 | 0.592 | -0.219 | 14.346 | 11.667 | 2.678 |
| 6.642 | 0.393 | 0.258 | 1.636 | 1.620 | 1.113 | 0.758 | -0.250 | 13.683 | 10.631 | 3.052 |
| 6.642 | 0.505 | 0.311 | 1.708 | 1.689 | 1.032 | 0.915 | -0.259 | 13.125 | 9.720 | 3.405 |
| 6.642 | 0.617 | 0.363 | 1.805 | 1.783 | 0.954 | 1.068 | -0.239 | 12.550 | 8.886 | 3.664 |
| 6.642 | 0.729 | 0.423 | 1.936 | 1.912 | 0.865 | 1.245 | -0.198 | 12.005 | 7.976 | 4.029 |
| 6.642 | 0.842 | 0.487 | 2.118 | 2.092 | 0.769 | 1.435 | -0.112 | 11.429 | 7.031 | 4.398 |
| 6.642 | 0.954 | 0.554 | 2.368 | 2.341 | 0.668 | 1.635 | 0.038 | 10.796 | 6.055 | 4.741 |
| 6.642 | 1.066 | 0.638 | 2.718 | 2.691 | 0.540 | 1.890 | 0.260 | 10.102 | 4.840 | 5.262 |
| 6.642 | 1.178 | 0.725 | 3.207 | 3.182 | 0.410 | 2.153 | 0.619 | 9.307 | 3.591 | 5.716 |
| 6.642 | 1.291 | 0.826 | 3.896 | 3.876 | 0.259 | 2.461 | 1.157 | 8.338 | 2.132 | 6.205 |
| 13.284 | 0.056 | 0.056 | 1.512 | 1.517 | 1.416 | 0.173 | -0.072 | 17.273 | 16.168 | 1.104 |
| 13.284 | 0.168 | 0.131 | 1.544 | 1.539 | 1.304 | 0.387 | -0.152 | 16.148 | 13.993 | 2.155 |
| 13.284 | 0.281 | 0.196 | 1.584 | 1.576 | 1.205 | 0.581 | -0.210 | 15.554 | 12.572 | 2.981 |
| 13.284 | 0.393 | 0.249 | 1.636 | 1.625 | 1.126 | 0.736 | -0.237 | 14.945 | 11.533 | 3.412 |
| 13.284 | 0.505 | 0.289 | 1.702 | 1.689 | 1.066 | 0.854 | -0.231 | 14.346 | 10.763 | 3.583 |
| 13.284 | 0.617 | 0.331 | 1.791 | 1.775 | 1.003 | 0.978 | -0.206 | 13.813 | 10.015 | 3.798 |
| 13.284 | 0.729 | 0.382 | 1.904 | 1.887 | 0.926 | 1.130 | -0.169 | 13.354 | 9.168 | 4.186 |
| 13.284 | 0.842 | 0.437 | 2.054 | 2.035 | 0.843 | 1.293 | -0.101 | 12.834 | 8.287 | 4.548 |
| 13.284 | 0.954 | 0.504 | 2.254 | 2.233 | 0.743 | 1.491 | -0.001 | 12.347 | 7.254 | 5.094 |
| 13.284 | 1.066 | 0.559 | 2.517 | 2.495 | 0.660 | 1.658 | 0.178 | 11.784 | 6.388 | 5.396 |
| 13.284 | 1.178 | 0.624 | 2.869 | 2.846 | 0.562 | 1.852 | 0.432 | 11.171 | 5.391 | 5.780 |
| 13.284 | 1.291 | 0.703 | 3.336 | 3.313 | 0.445 | 2.087 | 0.782 | 10.488 | 4.196 | 6.292 |
| 13.284 | 1.403 | 0.794 | 3.953 | 3.932 | 0.307 | 2.364 | 1.262 | 9.654 | 2.788 | 6.866 |
| 13.284 | 1.515 | 0.881 | 4.326 | 4.310 | 0.178 | 2.627 | 1.506 | 8.717 | 1.448 | 7.269 |
| 39.853 | 0.056 | 0.045 | 1.512 | 1.512 | 1.433 | 0.135 | -0.055 | 18.938 | 17.916 | 1.022 |
| 39.853 | 0.168 | 0.112 | 1.542 | 1.541 | 1.332 | 0.335 | -0.125 | 17.900 | 15.741 | 2.159 |
| 39.853 | 0.281 | 0.165 | 1.579 | 1.578 | 1.252 | 0.495 | -0.168 | 17.246 | 14.409 | 2.837 |
| 39.853 | 0.393 | 0.210 | 1.623 | 1.621 | 1.185 | 0.628 | -0.191 | 16.705 | 13.405 | 3.300 |
| 39.853 | 0.505 | 0.252 | 1.679 | 1.677 | 1.121 | 0.755 | -0.199 | 16.261 | 12.526 | 3.735 |
| 39.853 | 0.617 | 0.300 | 1.749 | 1.746 | 1.049 | 0.897 | -0.200 | 15.864 | 11.613 | 4.251 |
| 39.853 | 0.729 | 0.325 | 1.836 | 1.833 | 1.011 | 0.973 | -0.152 | 15.351 | 11.093 | 4.258 |
| 39.853 | 0.842 | 0.366 | 1.944 | 1.940 | 0.950 | 1.095 | -0.105 | 14.930 | 10.349 | 4.581 |
| 39.853 | 0.954 | 0.412 | 2.079 | 2.075 | 0.880 | 1.233 | -0.039 | 14.569 | 9.538 | 5.030 |
| 39.853 | 1.066 | 0.452 | 2.246 | 2.242 | 0.819 | 1.355 | 0.067 | 14.136 | 8.828 | 5.308 |
| 39.853 | 1.178 | 0.494 | 2.456 | 2.452 | 0.757 | 1.480 | 0.215 | 13.687 | 8.112 | 5.576 |
| 39.853 | 1.291 | 0.555 | 2.718 | 2.714 | 0.665 | 1.663 | 0.386 | 13.248 | 7.088 | 6.160 |
| 39.853 | 1.403 | 0.618 | 3.046 | 3.042 | 0.571 | 1.852 | 0.619 | 12.761 | 6.039 | 6.722 |
| 39.853 | 1.515 | 0.678 | 3.453 | 3.449 | 0.480 | 2.033 | 0.935 | 12.215 | 5.028 | 7.187 |
| 39.853 | 1.627 | 0.742 | 3.959 | 3.955 | 0.384 | 2.226 | 1.345 | 11.612 | 3.950 | 7.661 |
| 39.853 | 1.740 | 0.809 | 4.591 | 4.588 | 0.284 | 2.428 | 1.877 | 10.935 | 2.819 | 8.116 |
| 66.421 | 0.056 | 0.039 | 1.512 | 1.512 | 1.441 | 0.119 | -0.047 | 19.701 | 18.748 | 0.954 |
| 66.421 | 0.168 | 0.098 | 1.540 | 1.540 | 1.353 | 0.293 | -0.106 | 18.578 | 16.668 | 1.909 |
| 66.421 | 0.281 | 0.154 | 1.574 | 1.574 | 1.268 | 0.463 | -0.157 | 18.049 | 15.237 | 2.812 |
| 66.421 | 0.393 | 0.194 | 1.616 | 1.615 | 1.209 | 0.581 | -0.175 | 17.510 | 14.282 | 3.228 |
| 66.421 | 0.505 | 0.232 | 1.666 | 1.666 | 1.151 | 0.696 | -0.181 | 17.071 | 13.441 | 3.630 |
| 66.421 | 0.617 | 0.278 | 1.728 | 1.728 | 1.081 | 0.835 | -0.189 | 16.729 | 12.510 | 4.219 |
| 66.421 | 0.729 | 0.308 | 1.803 | 1.802 | 1.036 | 0.926 | -0.160 | 16.302 | 11.885 | 4.418 |
| 66.421 | 0.842 | 0.342 | 1.894 | 1.893 | 0.985 | 1.028 | -0.119 | 15.899 | 11.222 | 4.677 |
| 66.421 | 0.954 | 0.383 | 2.005 | 2.005 | 0.923 | 1.152 | -0.070 | 15.562 | 10.459 | 5.104 |

*Continued on next page*

TABLE S9 – Thermodynamic calculation results of repulsive 16-6 fluid (continued)

| $k_BT/\epsilon_{lj}$ | $\rho\sigma^3$ | $f_s$ | $E^{*,MD}$ | $E^{*,,tot}$ | $E^{*,g}$ | $E^{*,s}$ | $V_0^*$ | $S^{*,tot}$ | $S^{*,g}$ | $S^{*,s}$ |
|---|---|---|---|---|---|---|---|---|---|---|
| 66.421 | 1.066 | 0.422 | 2.142 | 2.141 | 0.865 | 1.267 | 0.009 | 15.183 | 9.752 | 5.431 |
| 66.421 | 1.178 | 0.460 | 2.307 | 2.307 | 0.808 | 1.382 | 0.117 | 14.788 | 9.060 | 5.728 |
| 66.421 | 1.291 | 0.510 | 2.511 | 2.511 | 0.732 | 1.533 | 0.246 | 14.399 | 8.177 | 6.221 |
| 66.421 | 1.403 | 0.552 | 2.760 | 2.760 | 0.669 | 1.659 | 0.432 | 13.974 | 7.432 | 6.542 |
| 66.421 | 1.515 | 0.609 | 3.063 | 3.063 | 0.584 | 1.829 | 0.650 | 13.532 | 6.447 | 7.085 |
| 66.421 | 1.627 | 0.664 | 3.431 | 3.431 | 0.501 | 1.995 | 0.935 | 13.045 | 5.484 | 7.562 |
| 66.421 | 1.740 | 0.715 | 3.876 | 3.877 | 0.424 | 2.149 | 1.304 | 12.507 | 4.588 | 7.918 |
| 66.421 | 1.852 | 0.777 | 4.420 | 4.421 | 0.330 | 2.337 | 1.753 | 11.930 | 3.495 | 8.435 |
| 66.421 | 1.964 | 0.838 | 5.081 | 5.083 | 0.240 | 2.519 | 2.324 | 11.281 | 2.431 | 8.850 |
| 92.989 | 0.056 | 0.037 | 1.511 | 1.512 | 1.444 | 0.112 | -0.044 | 20.162 | 19.274 | 0.888 |
| 92.989 | 0.168 | 0.095 | 1.539 | 1.539 | 1.357 | 0.286 | -0.104 | 19.135 | 17.171 | 1.964 |
| 92.989 | 0.281 | 0.145 | 1.571 | 1.572 | 1.282 | 0.435 | -0.146 | 18.563 | 15.828 | 2.736 |
| 92.989 | 0.393 | 0.189 | 1.610 | 1.610 | 1.215 | 0.569 | -0.174 | 18.101 | 14.763 | 3.338 |
| 92.989 | 0.505 | 0.224 | 1.657 | 1.657 | 1.162 | 0.675 | -0.180 | 17.652 | 13.949 | 3.702 |
| 92.989 | 0.617 | 0.261 | 1.714 | 1.714 | 1.107 | 0.784 | -0.177 | 17.247 | 13.172 | 4.075 |
| 92.989 | 0.729 | 0.291 | 1.781 | 1.782 | 1.062 | 0.875 | -0.155 | 16.861 | 12.527 | 4.333 |
| 92.989 | 0.842 | 0.324 | 1.864 | 1.865 | 1.012 | 0.974 | -0.122 | 16.492 | 11.864 | 4.628 |
| 92.989 | 0.954 | 0.365 | 1.962 | 1.963 | 0.950 | 1.099 | -0.086 | 16.195 | 11.076 | 5.119 |
| 92.989 | 1.066 | 0.402 | 2.082 | 2.083 | 0.894 | 1.210 | -0.022 | 15.838 | 10.374 | 5.463 |
| 92.989 | 1.178 | 0.432 | 2.225 | 2.226 | 0.850 | 1.299 | 0.078 | 15.454 | 9.812 | 5.641 |
| 92.989 | 1.291 | 0.471 | 2.398 | 2.400 | 0.790 | 1.418 | 0.192 | 15.094 | 9.086 | 6.009 |
| 92.989 | 1.403 | 0.522 | 2.607 | 2.608 | 0.713 | 1.572 | 0.323 | 14.737 | 8.163 | 6.574 |
| 92.989 | 1.515 | 0.564 | 2.856 | 2.858 | 0.651 | 1.696 | 0.511 | 14.330 | 7.418 | 6.912 |
| 92.989 | 1.627 | 0.611 | 3.158 | 3.160 | 0.580 | 1.838 | 0.742 | 13.903 | 6.572 | 7.331 |
| 92.989 | 1.740 | 0.664 | 3.519 | 3.521 | 0.500 | 1.997 | 1.023 | 13.443 | 5.626 | 7.817 |
| 92.989 | 1.852 | 0.725 | 3.951 | 3.953 | 0.408 | 2.183 | 1.363 | 12.934 | 4.521 | 8.413 |
| 92.989 | 1.964 | 0.771 | 4.471 | 4.474 | 0.339 | 2.320 | 1.814 | 12.397 | 3.701 | 8.696 |
| 92.989 | 2.076 | 0.825 | 5.090 | 5.094 | 0.257 | 2.484 | 2.352 | 11.813 | 2.716 | 9.097 |

TABLE S10: Thermodynamic calculation results of repulsive 12-6 fluid

| $k_BT/\epsilon_{lj}$ | $\rho\sigma^3$ | $f_s$ | $E^{*,MD}$ | $E^{*,tot}$ | $E^{*,g}$ | $E^{*,s}$ | $V_0^*$ | $S^{*,tot}$ | $S^{*,g}$ | $S^{*,s}$ |
|---|---|---|---|---|---|---|---|---|---|---|
| 1.328 | 0.056 | 0.068 | 1.514 | 1.515 | 1.397 | 0.207 | -0.089 | 13.839 | 12.743 | 1.097 |
| 1.328 | 0.168 | 0.161 | 1.551 | 1.520 | 1.258 | 0.452 | -0.191 | 12.668 | 10.631 | 2.038 |
| 1.328 | 0.281 | 0.227 | 1.602 | 1.556 | 1.159 | 0.636 | -0.238 | 11.787 | 9.445 | 2.342 |
| 1.328 | 0.393 | 0.293 | 1.673 | 1.615 | 1.060 | 0.822 | -0.267 | 11.108 | 8.440 | 2.668 |
| 1.328 | 0.505 | 0.343 | 1.773 | 1.706 | 0.985 | 0.963 | -0.241 | 10.377 | 7.704 | 2.673 |
| 1.328 | 0.617 | 0.420 | 1.916 | 1.840 | 0.869 | 1.185 | -0.214 | 9.801 | 6.714 | 3.087 |
| 1.328 | 0.729 | 0.494 | 2.122 | 2.042 | 0.758 | 1.402 | -0.118 | 9.107 | 5.789 | 3.319 |
| 1.328 | 0.842 | 0.577 | 2.427 | 2.346 | 0.632 | 1.653 | 0.061 | 8.374 | 4.766 | 3.609 |
| 1.328 | 0.954 | 0.680 | 2.877 | 2.803 | 0.478 | 1.969 | 0.356 | 7.520 | 3.523 | 3.997 |
| 6.642 | 0.056 | 0.047 | 1.515 | 1.514 | 1.429 | 0.141 | -0.056 | 16.197 | 15.309 | 0.888 |
| 6.642 | 0.168 | 0.120 | 1.554 | 1.549 | 1.320 | 0.355 | -0.126 | 15.064 | 13.240 | 1.824 |
| 6.642 | 0.281 | 0.188 | 1.603 | 1.596 | 1.216 | 0.560 | -0.180 | 14.523 | 11.839 | 2.684 |
| 6.642 | 0.393 | 0.239 | 1.667 | 1.658 | 1.139 | 0.711 | -0.192 | 13.928 | 10.874 | 3.055 |
| 6.642 | 0.505 | 0.296 | 1.750 | 1.739 | 1.055 | 0.878 | -0.193 | 13.449 | 9.924 | 3.525 |
| 6.642 | 0.617 | 0.331 | 1.857 | 1.845 | 1.001 | 0.984 | -0.140 | 12.887 | 9.305 | 3.582 |
| 6.642 | 0.729 | 0.379 | 1.997 | 1.984 | 0.930 | 1.125 | -0.071 | 12.418 | 8.558 | 3.860 |
| 6.642 | 0.842 | 0.421 | 2.180 | 2.166 | 0.866 | 1.251 | 0.049 | 11.896 | 7.909 | 3.987 |
| 6.642 | 0.954 | 0.488 | 2.419 | 2.404 | 0.765 | 1.452 | 0.187 | 11.457 | 6.935 | 4.522 |
| 6.642 | 1.066 | 0.546 | 2.731 | 2.717 | 0.677 | 1.628 | 0.412 | 10.946 | 6.091 | 4.855 |
| 6.642 | 1.178 | 0.601 | 3.139 | 3.125 | 0.594 | 1.795 | 0.736 | 10.384 | 5.294 | 5.090 |
| 6.642 | 1.291 | 0.673 | 3.667 | 3.655 | 0.487 | 2.011 | 1.158 | 9.782 | 4.278 | 5.504 |
| 6.642 | 1.403 | 0.747 | 4.346 | 4.337 | 0.375 | 2.237 | 1.725 | 9.113 | 3.217 | 5.896 |
| 13.284 | 0.056 | 0.044 | 1.515 | 1.515 | 1.434 | 0.132 | -0.051 | 17.252 | 16.354 | 0.897 |
| 13.284 | 0.168 | 0.107 | 1.552 | 1.549 | 1.339 | 0.318 | -0.108 | 16.137 | 14.353 | 1.784 |
| 13.284 | 0.281 | 0.167 | 1.598 | 1.593 | 1.248 | 0.498 | -0.153 | 15.602 | 13.002 | 2.599 |
| 13.284 | 0.393 | 0.212 | 1.656 | 1.650 | 1.182 | 0.630 | -0.162 | 15.036 | 12.075 | 2.961 |
| 13.284 | 0.505 | 0.262 | 1.727 | 1.720 | 1.106 | 0.779 | -0.165 | 14.646 | 11.152 | 3.495 |
| 13.284 | 0.617 | 0.297 | 1.818 | 1.809 | 1.053 | 0.884 | -0.128 | 14.177 | 10.495 | 3.682 |
| 13.284 | 0.729 | 0.338 | 1.931 | 1.921 | 0.991 | 1.006 | -0.076 | 13.754 | 9.796 | 3.959 |
| 13.284 | 0.842 | 0.376 | 2.072 | 2.062 | 0.934 | 1.119 | 0.008 | 13.326 | 9.159 | 4.167 |
| 13.284 | 0.954 | 0.414 | 2.251 | 2.240 | 0.876 | 1.234 | 0.129 | 12.909 | 8.531 | 4.378 |
| 13.284 | 1.066 | 0.469 | 2.475 | 2.463 | 0.794 | 1.398 | 0.271 | 12.525 | 7.682 | 4.843 |
| 13.284 | 1.178 | 0.519 | 2.754 | 2.742 | 0.719 | 1.548 | 0.476 | 12.112 | 6.915 | 5.197 |
| 13.284 | 1.291 | 0.567 | 3.103 | 3.091 | 0.647 | 1.691 | 0.753 | 11.657 | 6.184 | 5.472 |
| 13.284 | 1.403 | 0.627 | 3.534 | 3.521 | 0.556 | 1.872 | 1.093 | 11.175 | 5.271 | 5.904 |
| 13.284 | 1.515 | 0.678 | 4.064 | 4.052 | 0.479 | 2.027 | 1.546 | 10.661 | 4.491 | 6.170 |
| 13.284 | 1.627 | 0.733 | 4.711 | 4.700 | 0.398 | 2.190 | 2.112 | 10.113 | 3.667 | 6.445 |
| 39.853 | 0.056 | 0.035 | 1.513 | 1.513 | 1.448 | 0.104 | -0.038 | 18.925 | 18.098 | 0.827 |
| 39.853 | 0.168 | 0.092 | 1.546 | 1.546 | 1.361 | 0.278 | -0.092 | 17.946 | 16.063 | 1.884 |
| 39.853 | 0.281 | 0.135 | 1.585 | 1.585 | 1.296 | 0.406 | -0.117 | 17.314 | 14.900 | 2.414 |
| 39.853 | 0.393 | 0.182 | 1.632 | 1.632 | 1.226 | 0.547 | -0.141 | 16.894 | 13.851 | 3.044 |
| 39.853 | 0.505 | 0.215 | 1.687 | 1.687 | 1.175 | 0.647 | -0.136 | 16.477 | 13.109 | 3.368 |
| 39.853 | 0.617 | 0.245 | 1.753 | 1.753 | 1.131 | 0.737 | -0.114 | 16.071 | 12.478 | 3.593 |
| 39.853 | 0.729 | 0.281 | 1.832 | 1.832 | 1.076 | 0.846 | -0.089 | 15.758 | 11.778 | 3.979 |
| 39.853 | 0.842 | 0.311 | 1.926 | 1.927 | 1.030 | 0.938 | -0.041 | 15.421 | 11.194 | 4.227 |
| 39.853 | 0.954 | 0.346 | 2.038 | 2.039 | 0.978 | 1.042 | 0.019 | 15.112 | 10.563 | 4.549 |
| 39.853 | 1.066 | 0.370 | 2.172 | 2.173 | 0.941 | 1.115 | 0.117 | 14.756 | 10.109 | 4.647 |
| 39.853 | 1.178 | 0.411 | 2.330 | 2.331 | 0.880 | 1.237 | 0.214 | 14.471 | 9.412 | 5.059 |
| 39.853 | 1.291 | 0.449 | 2.518 | 2.519 | 0.822 | 1.353 | 0.344 | 14.167 | 8.752 | 5.415 |
| 39.853 | 1.403 | 0.476 | 2.739 | 2.741 | 0.782 | 1.433 | 0.526 | 13.813 | 8.286 | 5.528 |
| 39.853 | 1.515 | 0.519 | 3.000 | 3.002 | 0.716 | 1.564 | 0.721 | 13.500 | 7.559 | 5.942 |
| 39.853 | 1.627 | 0.555 | 3.305 | 3.307 | 0.663 | 1.671 | 0.973 | 13.151 | 6.964 | 6.187 |
| 39.853 | 1.740 | 0.595 | 3.663 | 3.665 | 0.602 | 1.793 | 1.270 | 12.792 | 6.290 | 6.502 |
| 39.853 | 1.852 | 0.634 | 4.078 | 4.081 | 0.543 | 1.911 | 1.627 | 12.416 | 5.639 | 6.777 |
| 39.853 | 1.964 | 0.681 | 4.557 | 4.560 | 0.473 | 2.052 | 2.035 | 12.021 | 4.865 | 7.156 |
| 39.853 | 2.076 | 0.725 | 5.110 | 5.113 | 0.406 | 2.185 | 2.522 | 11.603 | 4.134 | 7.470 |
| 66.421 | 0.056 | 0.030 | 1.513 | 1.513 | 1.454 | 0.092 | -0.033 | 19.675 | 18.912 | 0.762 |
| 66.421 | 0.168 | 0.080 | 1.543 | 1.544 | 1.379 | 0.241 | -0.077 | 18.628 | 16.975 | 1.653 |
| 66.421 | 0.281 | 0.127 | 1.579 | 1.580 | 1.308 | 0.384 | -0.112 | 18.160 | 15.691 | 2.469 |
| 66.421 | 0.393 | 0.165 | 1.620 | 1.621 | 1.251 | 0.498 | -0.127 | 17.716 | 14.757 | 2.959 |

*Continued on next page*

TABLE S10 – Thermodynamic calculation results of repulsive 12-6 fluid (continued)

| $k_BT/\epsilon_{lj}$ | $\rho\sigma^3$ | $f_s$ | $E^{*,MD}$ | $E^{*,tot}$ | $E^{*,g}$ | $E^{*,s}$ | $V_0^*$ | $S^{*,tot}$ | $S^{*,g}$ | $S^{*,s}$ |
|---|---|---|---|---|---|---|---|---|---|---|
| 66.421 | 0.505 | 0.202 | 1.669 | 1.670 | 1.195 | 0.609 | -0.134 | 17.359 | 13.931 | 3.428 |
| 66.421 | 0.617 | 0.229 | 1.725 | 1.727 | 1.154 | 0.691 | -0.118 | 16.981 | 13.316 | 3.665 |
| 66.421 | 0.729 | 0.263 | 1.792 | 1.794 | 1.102 | 0.795 | -0.103 | 16.705 | 12.617 | 4.088 |
| 66.421 | 0.842 | 0.284 | 1.869 | 1.872 | 1.070 | 0.859 | -0.057 | 16.334 | 12.160 | 4.174 |
| 66.421 | 0.954 | 0.311 | 1.960 | 1.963 | 1.030 | 0.938 | -0.006 | 16.026 | 11.639 | 4.387 |
| 66.421 | 1.066 | 0.337 | 2.066 | 2.069 | 0.991 | 1.018 | 0.061 | 15.726 | 11.130 | 4.596 |
| 66.421 | 1.178 | 0.367 | 2.189 | 2.192 | 0.944 | 1.110 | 0.138 | 15.465 | 10.560 | 4.905 |
| 66.421 | 1.291 | 0.398 | 2.332 | 2.336 | 0.898 | 1.203 | 0.235 | 15.198 | 9.999 | 5.199 |
| 66.421 | 1.403 | 0.435 | 2.498 | 2.502 | 0.842 | 1.315 | 0.345 | 14.941 | 9.343 | 5.598 |
| 66.421 | 1.515 | 0.458 | 2.689 | 2.694 | 0.807 | 1.384 | 0.502 | 14.627 | 8.923 | 5.704 |
| 66.421 | 1.627 | 0.492 | 2.911 | 2.915 | 0.757 | 1.485 | 0.673 | 14.340 | 8.332 | 6.008 |
| 66.421 | 1.740 | 0.523 | 3.165 | 3.170 | 0.710 | 1.579 | 0.881 | 14.042 | 7.785 | 6.256 |
| 66.421 | 1.852 | 0.558 | 3.457 | 3.462 | 0.657 | 1.685 | 1.120 | 13.736 | 7.179 | 6.557 |
| 66.421 | 1.964 | 0.591 | 3.790 | 3.796 | 0.606 | 1.786 | 1.403 | 13.415 | 6.597 | 6.818 |
| 66.421 | 2.076 | 0.624 | 4.169 | 4.175 | 0.557 | 1.885 | 1.733 | 13.086 | 6.032 | 7.054 |
| 66.421 | 2.188 | 0.669 | 4.599 | 4.606 | 0.489 | 2.021 | 2.096 | 12.743 | 5.254 | 7.489 |
| 66.421 | 2.301 | 0.704 | 5.085 | 5.092 | 0.436 | 2.127 | 2.529 | 12.382 | 4.650 | 7.732 |
| 66.421 | 2.413 | 0.745 | 5.634 | 5.642 | 0.375 | 2.250 | 3.017 | 11.999 | 3.949 | 8.050 |
| 92.989 | 0.056 | 0.029 | 1.512 | 1.513 | 1.456 | 0.088 | -0.031 | 20.246 | 19.424 | 0.822 |
| 92.989 | 0.168 | 0.075 | 1.541 | 1.542 | 1.386 | 0.227 | -0.072 | 19.176 | 17.525 | 1.651 |
| 92.989 | 0.281 | 0.120 | 1.574 | 1.575 | 1.318 | 0.363 | -0.107 | 18.687 | 16.253 | 2.434 |
| 92.989 | 0.393 | 0.153 | 1.612 | 1.614 | 1.268 | 0.464 | -0.117 | 18.233 | 15.377 | 2.856 |
| 92.989 | 0.505 | 0.189 | 1.657 | 1.659 | 1.214 | 0.571 | -0.126 | 17.908 | 14.553 | 3.355 |
| 92.989 | 0.617 | 0.215 | 1.708 | 1.711 | 1.175 | 0.649 | -0.114 | 17.523 | 13.942 | 3.581 |
| 92.989 | 0.729 | 0.239 | 1.767 | 1.770 | 1.138 | 0.723 | -0.091 | 17.192 | 13.398 | 3.794 |
| 92.989 | 0.842 | 0.266 | 1.836 | 1.839 | 1.097 | 0.806 | -0.063 | 16.909 | 12.823 | 4.087 |
| 92.989 | 0.954 | 0.292 | 1.914 | 1.918 | 1.057 | 0.885 | -0.024 | 16.634 | 12.288 | 4.346 |
| 92.989 | 1.066 | 0.315 | 2.006 | 2.010 | 1.022 | 0.955 | 0.032 | 16.343 | 11.815 | 4.529 |
| 92.989 | 1.178 | 0.350 | 2.110 | 2.115 | 0.970 | 1.059 | 0.086 | 16.138 | 11.169 | 4.969 |
| 92.989 | 1.291 | 0.371 | 2.231 | 2.236 | 0.939 | 1.122 | 0.175 | 15.850 | 10.758 | 5.092 |
| 92.989 | 1.403 | 0.399 | 2.369 | 2.374 | 0.895 | 1.210 | 0.270 | 15.597 | 10.218 | 5.379 |
| 92.989 | 1.515 | 0.420 | 2.527 | 2.533 | 0.863 | 1.272 | 0.397 | 15.312 | 9.822 | 5.489 |
| 92.989 | 1.627 | 0.448 | 2.708 | 2.714 | 0.822 | 1.356 | 0.536 | 15.046 | 9.316 | 5.730 |
| 92.989 | 1.740 | 0.478 | 2.913 | 2.920 | 0.777 | 1.446 | 0.697 | 14.789 | 8.776 | 6.014 |
| 92.989 | 1.852 | 0.515 | 3.147 | 3.154 | 0.720 | 1.560 | 0.874 | 14.533 | 8.108 | 6.426 |
| 92.989 | 1.964 | 0.546 | 3.411 | 3.419 | 0.674 | 1.652 | 1.093 | 14.262 | 7.562 | 6.700 |
| 92.989 | 2.076 | 0.580 | 3.710 | 3.718 | 0.621 | 1.757 | 1.339 | 13.972 | 6.944 | 7.028 |
| 92.989 | 2.188 | 0.615 | 4.047 | 4.055 | 0.568 | 1.863 | 1.624 | 13.673 | 6.327 | 7.346 |
| 92.989 | 2.301 | 0.646 | 4.425 | 4.433 | 0.522 | 1.956 | 1.955 | 13.357 | 5.776 | 7.580 |
| 92.989 | 2.413 | 0.682 | 4.848 | 4.857 | 0.468 | 2.063 | 2.325 | 13.034 | 5.151 | 7.883 |
| 92.989 | 2.525 | 0.713 | 5.321 | 5.331 | 0.422 | 2.157 | 2.752 | 12.697 | 4.602 | 8.095 |

TABLE S11: Thermodynamic calculation results of repulsive 8-6 fluid

| $k_BT/\epsilon_{lj}$ | $\rho\sigma^3$ | $f_s$ | $E^{*,MD}$ | $E^{*,tot}$ | $E^{*,g}$ | $E^{*,s}$ | $V_0^*$ | $S^{*,tot}$ | $S^{*,g}$ | $S^{*,s}$ |
|---|---|---|---|---|---|---|---|---|---|---|
| 1.328 | 0.056 | 0.057 | 1.519 | 1.521 | 1.414 | 0.174 | -0.067 | 13.878 | 12.887 | 0.991 |
| 1.328 | 0.168 | 0.138 | 1.567 | 1.538 | 1.292 | 0.387 | -0.141 | 12.821 | 10.897 | 1.925 |
| 1.328 | 0.281 | 0.198 | 1.629 | 1.585 | 1.203 | 0.550 | -0.167 | 12.055 | 9.783 | 2.271 |
| 1.328 | 0.393 | 0.254 | 1.712 | 1.655 | 1.119 | 0.705 | -0.168 | 11.490 | 8.885 | 2.605 |
| 1.328 | 0.505 | 0.301 | 1.822 | 1.755 | 1.048 | 0.836 | -0.129 | 10.931 | 8.175 | 2.756 |
| 1.328 | 0.617 | 0.355 | 1.968 | 1.891 | 0.967 | 0.988 | -0.064 | 10.463 | 7.443 | 3.021 |
| 1.328 | 0.729 | 0.400 | 2.164 | 2.079 | 0.899 | 1.115 | 0.064 | 9.943 | 6.841 | 3.102 |
| 1.328 | 0.842 | 0.462 | 2.424 | 2.331 | 0.806 | 1.294 | 0.231 | 9.462 | 6.071 | 3.391 |
| 1.328 | 0.954 | 0.514 | 2.768 | 2.671 | 0.728 | 1.446 | 0.497 | 8.954 | 5.428 | 3.526 |
| 1.328 | 1.066 | 0.567 | 3.223 | 3.125 | 0.648 | 1.603 | 0.873 | 8.427 | 4.786 | 3.641 |
| 1.328 | 1.178 | 0.635 | 3.815 | 3.717 | 0.546 | 1.809 | 1.363 | 7.876 | 3.976 | 3.901 |
| 6.642 | 0.056 | 0.035 | 1.517 | 1.516 | 1.447 | 0.106 | -0.036 | 16.223 | 15.491 | 0.732 |
| 6.642 | 0.168 | 0.093 | 1.560 | 1.556 | 1.360 | 0.275 | -0.079 | 15.214 | 13.621 | 1.594 |
| 6.642 | 0.281 | 0.139 | 1.610 | 1.604 | 1.291 | 0.411 | -0.098 | 14.639 | 12.529 | 2.110 |
| 6.642 | 0.393 | 0.185 | 1.672 | 1.664 | 1.221 | 0.548 | -0.106 | 14.239 | 11.612 | 2.627 |
| 6.642 | 0.505 | 0.216 | 1.746 | 1.737 | 1.174 | 0.642 | -0.079 | 13.764 | 10.987 | 2.776 |
| 6.642 | 0.617 | 0.258 | 1.835 | 1.824 | 1.112 | 0.763 | -0.051 | 13.473 | 10.287 | 3.186 |
| 6.642 | 0.729 | 0.286 | 1.943 | 1.930 | 1.069 | 0.847 | 0.014 | 13.103 | 9.793 | 3.309 |
| 6.642 | 0.842 | 0.313 | 2.071 | 2.058 | 1.028 | 0.929 | 0.101 | 12.764 | 9.329 | 3.435 |
| 6.642 | 0.954 | 0.339 | 2.227 | 2.212 | 0.990 | 1.004 | 0.219 | 12.408 | 8.914 | 3.494 |
| 6.642 | 1.066 | 0.377 | 2.410 | 2.395 | 0.932 | 1.119 | 0.344 | 12.146 | 8.340 | 3.806 |
| 6.642 | 1.178 | 0.407 | 2.628 | 2.612 | 0.886 | 1.209 | 0.517 | 11.844 | 7.883 | 3.961 |
| 6.642 | 1.291 | 0.441 | 2.885 | 2.868 | 0.835 | 1.310 | 0.723 | 11.555 | 7.388 | 4.166 |
| 6.642 | 1.403 | 0.470 | 3.184 | 3.167 | 0.791 | 1.398 | 0.978 | 11.241 | 6.963 | 4.278 |
| 6.642 | 1.515 | 0.511 | 3.533 | 3.516 | 0.730 | 1.520 | 1.266 | 10.968 | 6.391 | 4.577 |
| 6.642 | 1.627 | 0.539 | 3.935 | 3.918 | 0.688 | 1.603 | 1.627 | 10.639 | 5.994 | 4.644 |
| 13.284 | 0.056 | 0.032 | 1.516 | 1.516 | 1.452 | 0.095 | -0.031 | 17.285 | 16.555 | 0.731 |
| 13.284 | 0.168 | 0.079 | 1.554 | 1.551 | 1.381 | 0.235 | -0.065 | 16.283 | 14.777 | 1.506 |
| 13.284 | 0.281 | 0.119 | 1.598 | 1.594 | 1.321 | 0.353 | -0.080 | 15.729 | 13.720 | 2.009 |
| 13.284 | 0.393 | 0.155 | 1.650 | 1.645 | 1.267 | 0.460 | -0.082 | 15.316 | 12.904 | 2.413 |
| 13.284 | 0.505 | 0.195 | 1.710 | 1.703 | 1.207 | 0.579 | -0.082 | 15.062 | 12.117 | 2.945 |
| 13.284 | 0.617 | 0.223 | 1.780 | 1.773 | 1.165 | 0.661 | -0.054 | 14.705 | 11.561 | 3.143 |
| 13.284 | 0.729 | 0.249 | 1.862 | 1.853 | 1.125 | 0.740 | -0.012 | 14.399 | 11.060 | 3.339 |
| 13.284 | 0.842 | 0.274 | 1.957 | 1.947 | 1.087 | 0.815 | 0.045 | 14.109 | 10.600 | 3.509 |
| 13.284 | 0.954 | 0.291 | 2.067 | 2.057 | 1.061 | 0.866 | 0.130 | 13.781 | 10.267 | 3.514 |
| 13.284 | 1.066 | 0.318 | 2.194 | 2.183 | 1.021 | 0.946 | 0.216 | 13.548 | 9.817 | 3.731 |
| 13.284 | 1.178 | 0.340 | 2.340 | 2.328 | 0.988 | 1.010 | 0.330 | 13.274 | 9.448 | 3.827 |
| 13.284 | 1.291 | 0.365 | 2.506 | 2.494 | 0.950 | 1.086 | 0.458 | 13.023 | 9.036 | 3.987 |
| 13.284 | 1.403 | 0.384 | 2.697 | 2.684 | 0.922 | 1.142 | 0.621 | 12.782 | 8.724 | 4.058 |
| 13.284 | 1.515 | 0.415 | 2.913 | 2.899 | 0.875 | 1.235 | 0.790 | 12.562 | 8.249 | 4.314 |
| 13.284 | 1.627 | 0.446 | 3.156 | 3.142 | 0.829 | 1.326 | 0.988 | 12.340 | 7.785 | 4.555 |
| 13.284 | 1.740 | 0.465 | 3.430 | 3.416 | 0.800 | 1.383 | 1.233 | 12.090 | 7.485 | 4.605 |
| 13.284 | 1.852 | 0.497 | 3.737 | 3.722 | 0.751 | 1.481 | 1.490 | 11.870 | 6.997 | 4.874 |
| 13.284 | 1.964 | 0.529 | 4.077 | 4.062 | 0.703 | 1.576 | 1.783 | 11.644 | 6.527 | 5.118 |
| 13.284 | 2.076 | 0.557 | 4.456 | 4.441 | 0.662 | 1.658 | 2.121 | 11.400 | 6.117 | 5.283 |
| 39.853 | 0.056 | 0.022 | 1.513 | 1.513 | 1.467 | 0.065 | -0.019 | 18.903 | 18.330 | 0.573 |
| 39.853 | 0.168 | 0.057 | 1.544 | 1.544 | 1.414 | 0.172 | -0.042 | 17.872 | 16.660 | 1.212 |
| 39.853 | 0.281 | 0.089 | 1.577 | 1.577 | 1.365 | 0.269 | -0.057 | 17.399 | 15.649 | 1.750 |
| 39.853 | 0.393 | 0.125 | 1.615 | 1.615 | 1.311 | 0.378 | -0.073 | 17.173 | 14.760 | 2.413 |
| 39.853 | 0.505 | 0.145 | 1.658 | 1.658 | 1.281 | 0.436 | -0.060 | 16.773 | 14.231 | 2.542 |
| 39.853 | 0.617 | 0.174 | 1.705 | 1.705 | 1.237 | 0.524 | -0.056 | 16.568 | 13.601 | 2.967 |
| 39.853 | 0.729 | 0.192 | 1.758 | 1.758 | 1.210 | 0.577 | -0.030 | 16.263 | 13.185 | 3.077 |
| 39.853 | 0.842 | 0.218 | 1.816 | 1.816 | 1.170 | 0.657 | -0.011 | 16.104 | 12.656 | 3.449 |
| 39.853 | 0.954 | 0.235 | 1.882 | 1.882 | 1.144 | 0.709 | 0.029 | 15.851 | 12.292 | 3.560 |
| 39.853 | 1.066 | 0.249 | 1.954 | 1.955 | 1.124 | 0.750 | 0.081 | 15.607 | 11.997 | 3.610 |
| 39.853 | 1.178 | 0.268 | 2.035 | 2.035 | 1.096 | 0.806 | 0.133 | 15.410 | 11.634 | 3.776 |
| 39.853 | 1.291 | 0.288 | 2.123 | 2.123 | 1.065 | 0.868 | 0.190 | 15.242 | 11.254 | 3.988 |
| 39.853 | 1.403 | 0.308 | 2.221 | 2.221 | 1.035 | 0.928 | 0.259 | 15.073 | 10.890 | 4.182 |
| 39.853 | 1.515 | 0.312 | 2.328 | 2.329 | 1.028 | 0.941 | 0.360 | 14.801 | 10.770 | 4.031 |
| 39.853 | 1.627 | 0.333 | 2.446 | 2.446 | 0.997 | 1.003 | 0.446 | 14.648 | 10.408 | 4.240 |

*Continued on next page*

TABLE S11 – Thermodynamic calculation results of repulsive 8-6 fluid (continued)

| $k_BT/\epsilon_{lj}$ | $\rho\sigma^3$ | $f_s$ | $E^{*,MD}$ | $E^{*,tot}$ | $E^{*,g}$ | $E^{*,s}$ | $V_0^*$ | $S^{*,tot}$ | $S^{*,g}$ | $S^{*,s}$ |
|---|---|---|---|---|---|---|---|---|---|---|
| 39.853 | 1.740 | 0.349 | 2.574 | 2.575 | 0.972 | 1.053 | 0.550 | 14.482 | 10.113 | 4.369 |
| 39.853 | 1.852 | 0.375 | 2.714 | 2.715 | 0.933 | 1.130 | 0.652 | 14.367 | 9.684 | 4.683 |
| 39.853 | 1.964 | 0.386 | 2.867 | 2.868 | 0.916 | 1.164 | 0.788 | 14.152 | 9.475 | 4.677 |
| 39.853 | 2.076 | 0.404 | 3.033 | 3.034 | 0.889 | 1.218 | 0.927 | 14.008 | 9.169 | 4.839 |
| 39.853 | 2.188 | 0.417 | 3.211 | 3.212 | 0.869 | 1.258 | 1.085 | 13.826 | 8.936 | 4.889 |
| 39.853 | 2.301 | 0.433 | 3.405 | 3.406 | 0.845 | 1.305 | 1.256 | 13.659 | 8.670 | 4.989 |
| 39.853 | 2.413 | 0.456 | 3.615 | 3.616 | 0.811 | 1.375 | 1.430 | 13.510 | 8.292 | 5.218 |
| 39.853 | 2.525 | 0.477 | 3.839 | 3.840 | 0.779 | 1.437 | 1.623 | 13.361 | 7.954 | 5.407 |
| 39.853 | 2.637 | 0.489 | 4.080 | 4.081 | 0.761 | 1.474 | 1.846 | 13.180 | 7.747 | 5.433 |
| 39.853 | 2.750 | 0.512 | 4.338 | 4.340 | 0.727 | 1.542 | 2.071 | 13.026 | 7.381 | 5.645 |
| 39.853 | 2.862 | 0.528 | 4.614 | 4.616 | 0.701 | 1.593 | 2.321 | 12.858 | 7.104 | 5.753 |
| 39.853 | 2.974 | 0.547 | 4.907 | 4.909 | 0.673 | 1.650 | 2.586 | 12.693 | 6.797 | 5.896 |
| 66.421 | 0.056 | 0.019 | 1.512 | 1.512 | 1.472 | 0.057 | -0.016 | 19.639 | 19.131 | 0.508 |
| 66.421 | 0.168 | 0.051 | 1.539 | 1.539 | 1.423 | 0.153 | -0.038 | 18.709 | 17.490 | 1.219 |
| 66.421 | 0.281 | 0.078 | 1.568 | 1.569 | 1.381 | 0.237 | -0.050 | 18.214 | 16.531 | 1.683 |
| 66.421 | 0.393 | 0.104 | 1.601 | 1.602 | 1.343 | 0.314 | -0.055 | 17.849 | 15.791 | 2.059 |
| 66.421 | 0.505 | 0.128 | 1.636 | 1.637 | 1.306 | 0.387 | -0.056 | 17.598 | 15.160 | 2.438 |
| 66.421 | 0.617 | 0.155 | 1.675 | 1.677 | 1.266 | 0.468 | -0.057 | 17.424 | 14.543 | 2.881 |
| 66.421 | 0.729 | 0.172 | 1.719 | 1.720 | 1.239 | 0.521 | -0.040 | 17.153 | 14.113 | 3.040 |
| 66.421 | 0.842 | 0.190 | 1.766 | 1.768 | 1.213 | 0.574 | -0.019 | 16.912 | 13.711 | 3.201 |
| 66.421 | 0.954 | 0.208 | 1.818 | 1.820 | 1.185 | 0.630 | 0.006 | 16.739 | 13.310 | 3.429 |
| 66.421 | 1.066 | 0.232 | 1.874 | 1.876 | 1.148 | 0.703 | 0.025 | 16.615 | 12.830 | 3.785 |
| 66.421 | 1.178 | 0.243 | 1.936 | 1.939 | 1.132 | 0.735 | 0.072 | 16.379 | 12.582 | 3.797 |
| 66.421 | 1.291 | 0.257 | 2.003 | 2.006 | 1.111 | 0.776 | 0.118 | 16.185 | 12.293 | 3.892 |
| 66.421 | 1.403 | 0.269 | 2.077 | 2.079 | 1.092 | 0.814 | 0.173 | 15.995 | 12.034 | 3.962 |
| 66.421 | 1.515 | 0.280 | 2.155 | 2.158 | 1.076 | 0.847 | 0.235 | 15.802 | 11.801 | 4.001 |
| 66.421 | 1.627 | 0.292 | 2.242 | 2.245 | 1.057 | 0.884 | 0.303 | 15.626 | 11.555 | 4.071 |
| 66.421 | 1.740 | 0.311 | 2.335 | 2.338 | 1.029 | 0.941 | 0.368 | 15.508 | 11.207 | 4.301 |
| 66.421 | 1.852 | 0.327 | 2.434 | 2.438 | 1.004 | 0.990 | 0.444 | 15.373 | 10.911 | 4.463 |
| 66.421 | 1.964 | 0.338 | 2.543 | 2.547 | 0.989 | 1.021 | 0.537 | 15.198 | 10.704 | 4.493 |
| 66.421 | 2.076 | 0.349 | 2.659 | 2.663 | 0.971 | 1.056 | 0.635 | 15.037 | 10.485 | 4.552 |
| 66.421 | 2.188 | 0.358 | 2.784 | 2.788 | 0.958 | 1.083 | 0.747 | 14.871 | 10.311 | 4.560 |
| 66.421 | 2.301 | 0.374 | 2.918 | 2.922 | 0.934 | 1.131 | 0.857 | 14.746 | 10.029 | 4.718 |
| 66.421 | 2.413 | 0.394 | 3.060 | 3.065 | 0.903 | 1.193 | 0.969 | 14.635 | 9.677 | 4.958 |
| 66.421 | 2.525 | 0.407 | 3.213 | 3.217 | 0.883 | 1.233 | 1.102 | 14.485 | 9.441 | 5.044 |
| 66.421 | 2.637 | 0.419 | 3.375 | 3.380 | 0.866 | 1.267 | 1.248 | 14.347 | 9.237 | 5.111 |
| 66.421 | 2.750 | 0.439 | 3.549 | 3.554 | 0.835 | 1.328 | 1.391 | 14.224 | 8.894 | 5.331 |
| 66.421 | 2.862 | 0.454 | 3.733 | 3.738 | 0.812 | 1.375 | 1.551 | 14.094 | 8.625 | 5.469 |
| 66.421 | 2.974 | 0.465 | 3.928 | 3.934 | 0.795 | 1.409 | 1.730 | 13.944 | 8.428 | 5.516 |
| 66.421 | 3.086 | 0.484 | 4.135 | 4.140 | 0.766 | 1.466 | 1.908 | 13.825 | 8.111 | 5.714 |
| 66.421 | 3.198 | 0.501 | 4.353 | 4.359 | 0.741 | 1.517 | 2.101 | 13.696 | 7.826 | 5.870 |
| 66.421 | 3.311 | 0.507 | 4.584 | 4.591 | 0.732 | 1.534 | 2.324 | 13.536 | 7.716 | 5.820 |
| 66.421 | 3.423 | 0.529 | 4.828 | 4.834 | 0.698 | 1.602 | 2.534 | 13.411 | 7.346 | 6.066 |
| 66.421 | 3.535 | 0.541 | 5.085 | 5.092 | 0.681 | 1.637 | 2.774 | 13.268 | 7.147 | 6.121 |
| 92.989 | 0.056 | 0.017 | 1.511 | 1.511 | 1.474 | 0.052 | -0.015 | 20.191 | 19.657 | 0.535 |
| 92.989 | 0.168 | 0.045 | 1.535 | 1.536 | 1.431 | 0.137 | -0.033 | 19.201 | 18.066 | 1.134 |
| 92.989 | 0.281 | 0.070 | 1.562 | 1.563 | 1.393 | 0.213 | -0.043 | 18.675 | 17.135 | 1.540 |
| 92.989 | 0.393 | 0.094 | 1.591 | 1.593 | 1.357 | 0.286 | -0.050 | 18.365 | 16.403 | 1.962 |
| 92.989 | 0.505 | 0.120 | 1.623 | 1.625 | 1.319 | 0.363 | -0.056 | 18.164 | 15.741 | 2.423 |
| 92.989 | 0.617 | 0.140 | 1.658 | 1.660 | 1.288 | 0.423 | -0.051 | 17.912 | 15.223 | 2.689 |
| 92.989 | 0.729 | 0.161 | 1.696 | 1.698 | 1.256 | 0.488 | -0.046 | 17.736 | 14.717 | 3.019 |
| 92.989 | 0.842 | 0.176 | 1.737 | 1.739 | 1.233 | 0.534 | -0.028 | 17.507 | 14.340 | 3.166 |
| 92.989 | 0.954 | 0.195 | 1.781 | 1.784 | 1.205 | 0.590 | -0.010 | 17.329 | 13.930 | 3.399 |
| 92.989 | 1.066 | 0.208 | 1.830 | 1.833 | 1.185 | 0.630 | 0.018 | 17.119 | 13.622 | 3.496 |
| 92.989 | 1.178 | 0.219 | 1.882 | 1.885 | 1.168 | 0.664 | 0.053 | 16.911 | 13.354 | 3.557 |
| 92.989 | 1.291 | 0.241 | 1.938 | 1.942 | 1.135 | 0.730 | 0.077 | 16.817 | 12.925 | 3.893 |
| 92.989 | 1.403 | 0.254 | 1.999 | 2.003 | 1.114 | 0.772 | 0.118 | 16.655 | 12.633 | 4.022 |
| 92.989 | 1.515 | 0.266 | 2.065 | 2.069 | 1.096 | 0.807 | 0.166 | 16.484 | 12.382 | 4.102 |
| 92.989 | 1.627 | 0.276 | 2.135 | 2.139 | 1.081 | 0.837 | 0.222 | 16.311 | 12.172 | 4.140 |
| 92.989 | 1.740 | 0.294 | 2.211 | 2.215 | 1.054 | 0.891 | 0.270 | 16.200 | 11.829 | 4.371 |
| 92.989 | 1.852 | 0.300 | 2.292 | 2.297 | 1.044 | 0.911 | 0.342 | 16.021 | 11.675 | 4.345 |

*Continued on next page*

TABLE S11 – Thermodynamic calculation results of repulsive 8-6 fluid (continued)

| $k_BT/\epsilon_{lj}$ | $\rho\sigma^3$ | $f_s$ | $E^{*,MD}$ | $E^{*,tot}$ | $E^{*,g}$ | $E^{*,s}$ | $V_0^*$ | $S^{*,tot}$ | $S^{*,g}$ | $S^{*,s}$ |
|---|---|---|---|---|---|---|---|---|---|---|
| 92.989 | 1.964 | 0.314 | 2.379 | 2.384 | 1.023 | 0.952 | 0.408 | 15.879 | 11.413 | 4.466 |
| 92.989 | 2.076 | 0.326 | 2.472 | 2.477 | 1.004 | 0.990 | 0.482 | 15.741 | 11.172 | 4.569 |
| 92.989 | 2.188 | 0.328 | 2.571 | 2.576 | 1.002 | 0.996 | 0.579 | 15.552 | 11.105 | 4.446 |
| 92.989 | 2.301 | 0.351 | 2.677 | 2.682 | 0.967 | 1.065 | 0.650 | 15.475 | 10.701 | 4.774 |
| 92.989 | 2.413 | 0.363 | 2.789 | 2.795 | 0.948 | 1.103 | 0.744 | 15.352 | 10.469 | 4.884 |
| 92.989 | 2.525 | 0.370 | 2.909 | 2.915 | 0.937 | 1.124 | 0.853 | 15.192 | 10.323 | 4.869 |
| 92.989 | 2.637 | 0.378 | 3.035 | 3.042 | 0.926 | 1.146 | 0.969 | 15.034 | 10.181 | 4.854 |
| 92.989 | 2.750 | 0.397 | 3.170 | 3.177 | 0.897 | 1.206 | 1.075 | 14.959 | 9.835 | 5.124 |
| 92.989 | 2.862 | 0.419 | 3.313 | 3.320 | 0.863 | 1.273 | 1.184 | 14.872 | 9.451 | 5.421 |
| 92.989 | 2.974 | 0.417 | 3.464 | 3.471 | 0.867 | 1.265 | 1.339 | 14.688 | 9.474 | 5.213 |
| 92.989 | 3.086 | 0.437 | 3.622 | 3.630 | 0.836 | 1.326 | 1.467 | 14.595 | 9.123 | 5.471 |
| 92.989 | 3.198 | 0.448 | 3.790 | 3.797 | 0.819 | 1.360 | 1.618 | 14.466 | 8.922 | 5.544 |
| 92.989 | 3.311 | 0.464 | 3.967 | 3.975 | 0.795 | 1.409 | 1.771 | 14.357 | 8.639 | 5.718 |
| 92.989 | 3.423 | 0.479 | 4.153 | 4.161 | 0.773 | 1.453 | 1.935 | 14.243 | 8.385 | 5.857 |
| 92.989 | 3.535 | 0.494 | 4.348 | 4.357 | 0.750 | 1.500 | 2.107 | 14.121 | 8.121 | 5.999 |
| 92.989 | 3.647 | 0.501 | 4.553 | 4.561 | 0.739 | 1.522 | 2.301 | 13.986 | 7.986 | 6.000 |
| 92.989 | 3.760 | 0.511 | 4.767 | 4.776 | 0.724 | 1.551 | 2.501 | 13.858 | 7.816 | 6.042 |
| 92.989 | 3.872 | 0.534 | 4.991 | 5.000 | 0.690 | 1.620 | 2.691 | 13.755 | 7.429 | 6.326 |
| 92.989 | 3.984 | 0.550 | 5.228 | 5.237 | 0.665 | 1.669 | 2.903 | 13.634 | 7.150 | 6.484 |
